# Supplementary material for: SFS: Smart OS Scheduling for Serverless Functions
Source: arXiv:2209.01709 source file (2022-09-07)
Supplement: Supplementary file 1 [file appendix.tex]

\if 0
\section{Appendix}

\subsection{CPU Scheduling Visualization (Visualized using Kernel Shark)}

\begin{figure}[h]
%\vspace{-5pt}
\begin{center}
\subfigure[CFS.] {
\includegraphics[width=.46\textwidth]{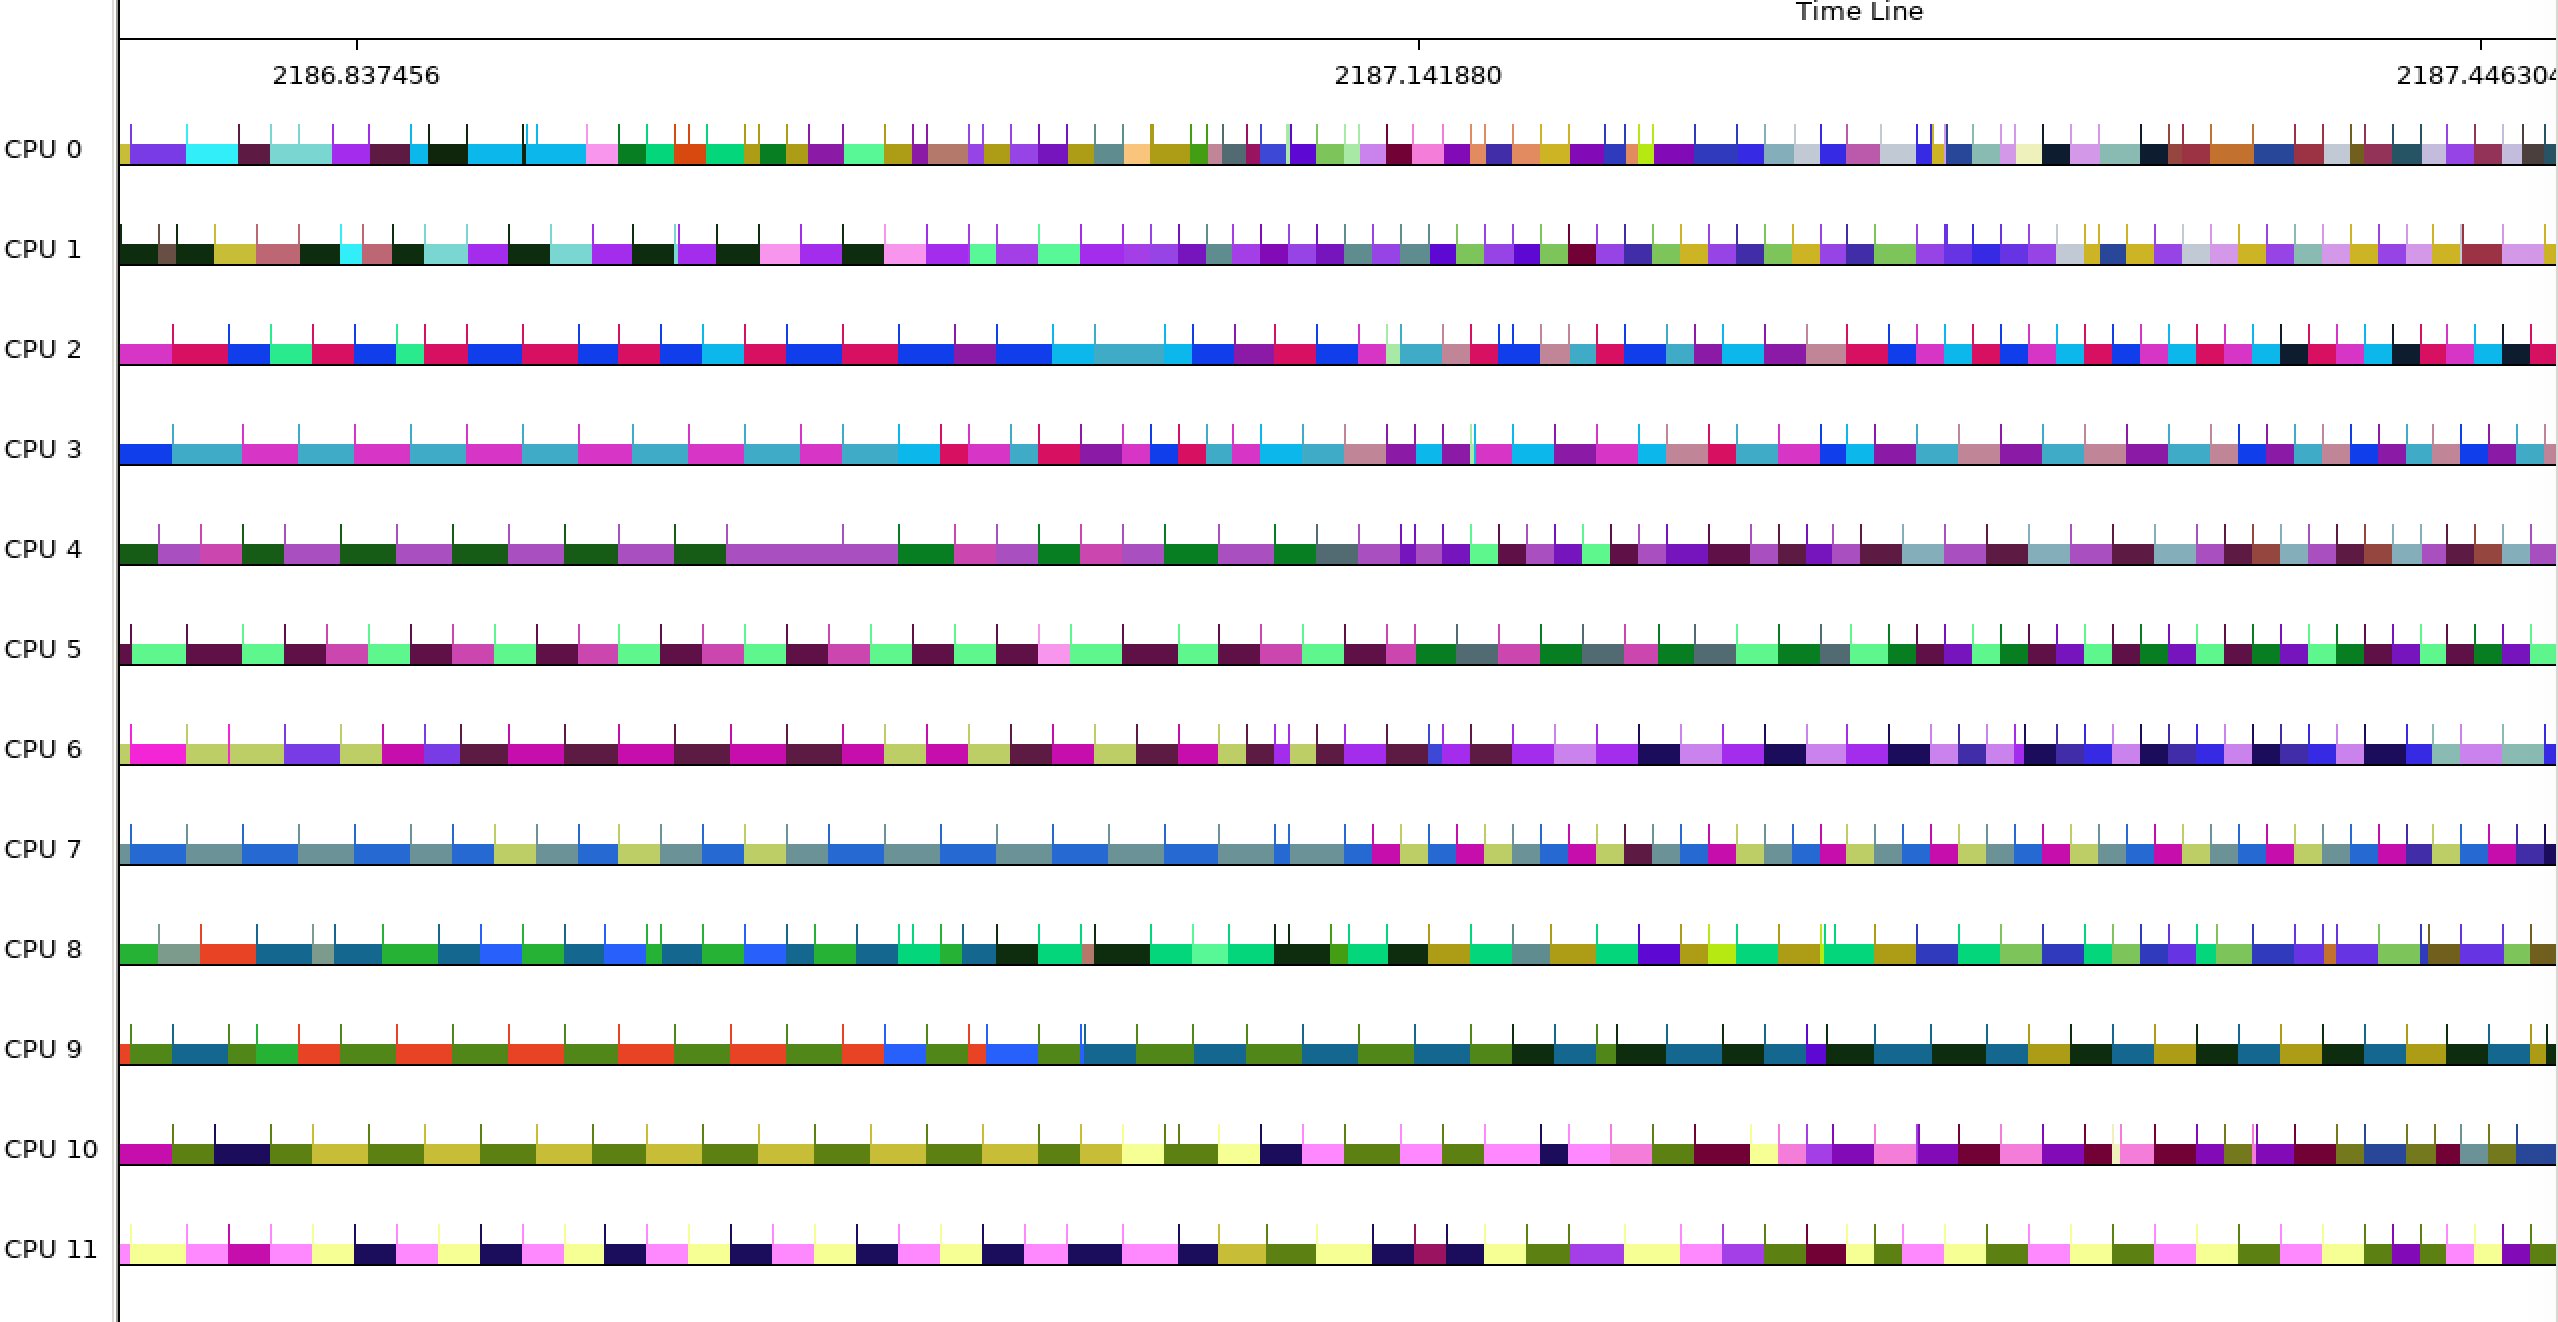}
\label{fig:kernel_cfs}
}
\hspace{4pt}
%\vspace{-20pt}
\subfigure[{\proj}.] {
\includegraphics[width=.48\textwidth]{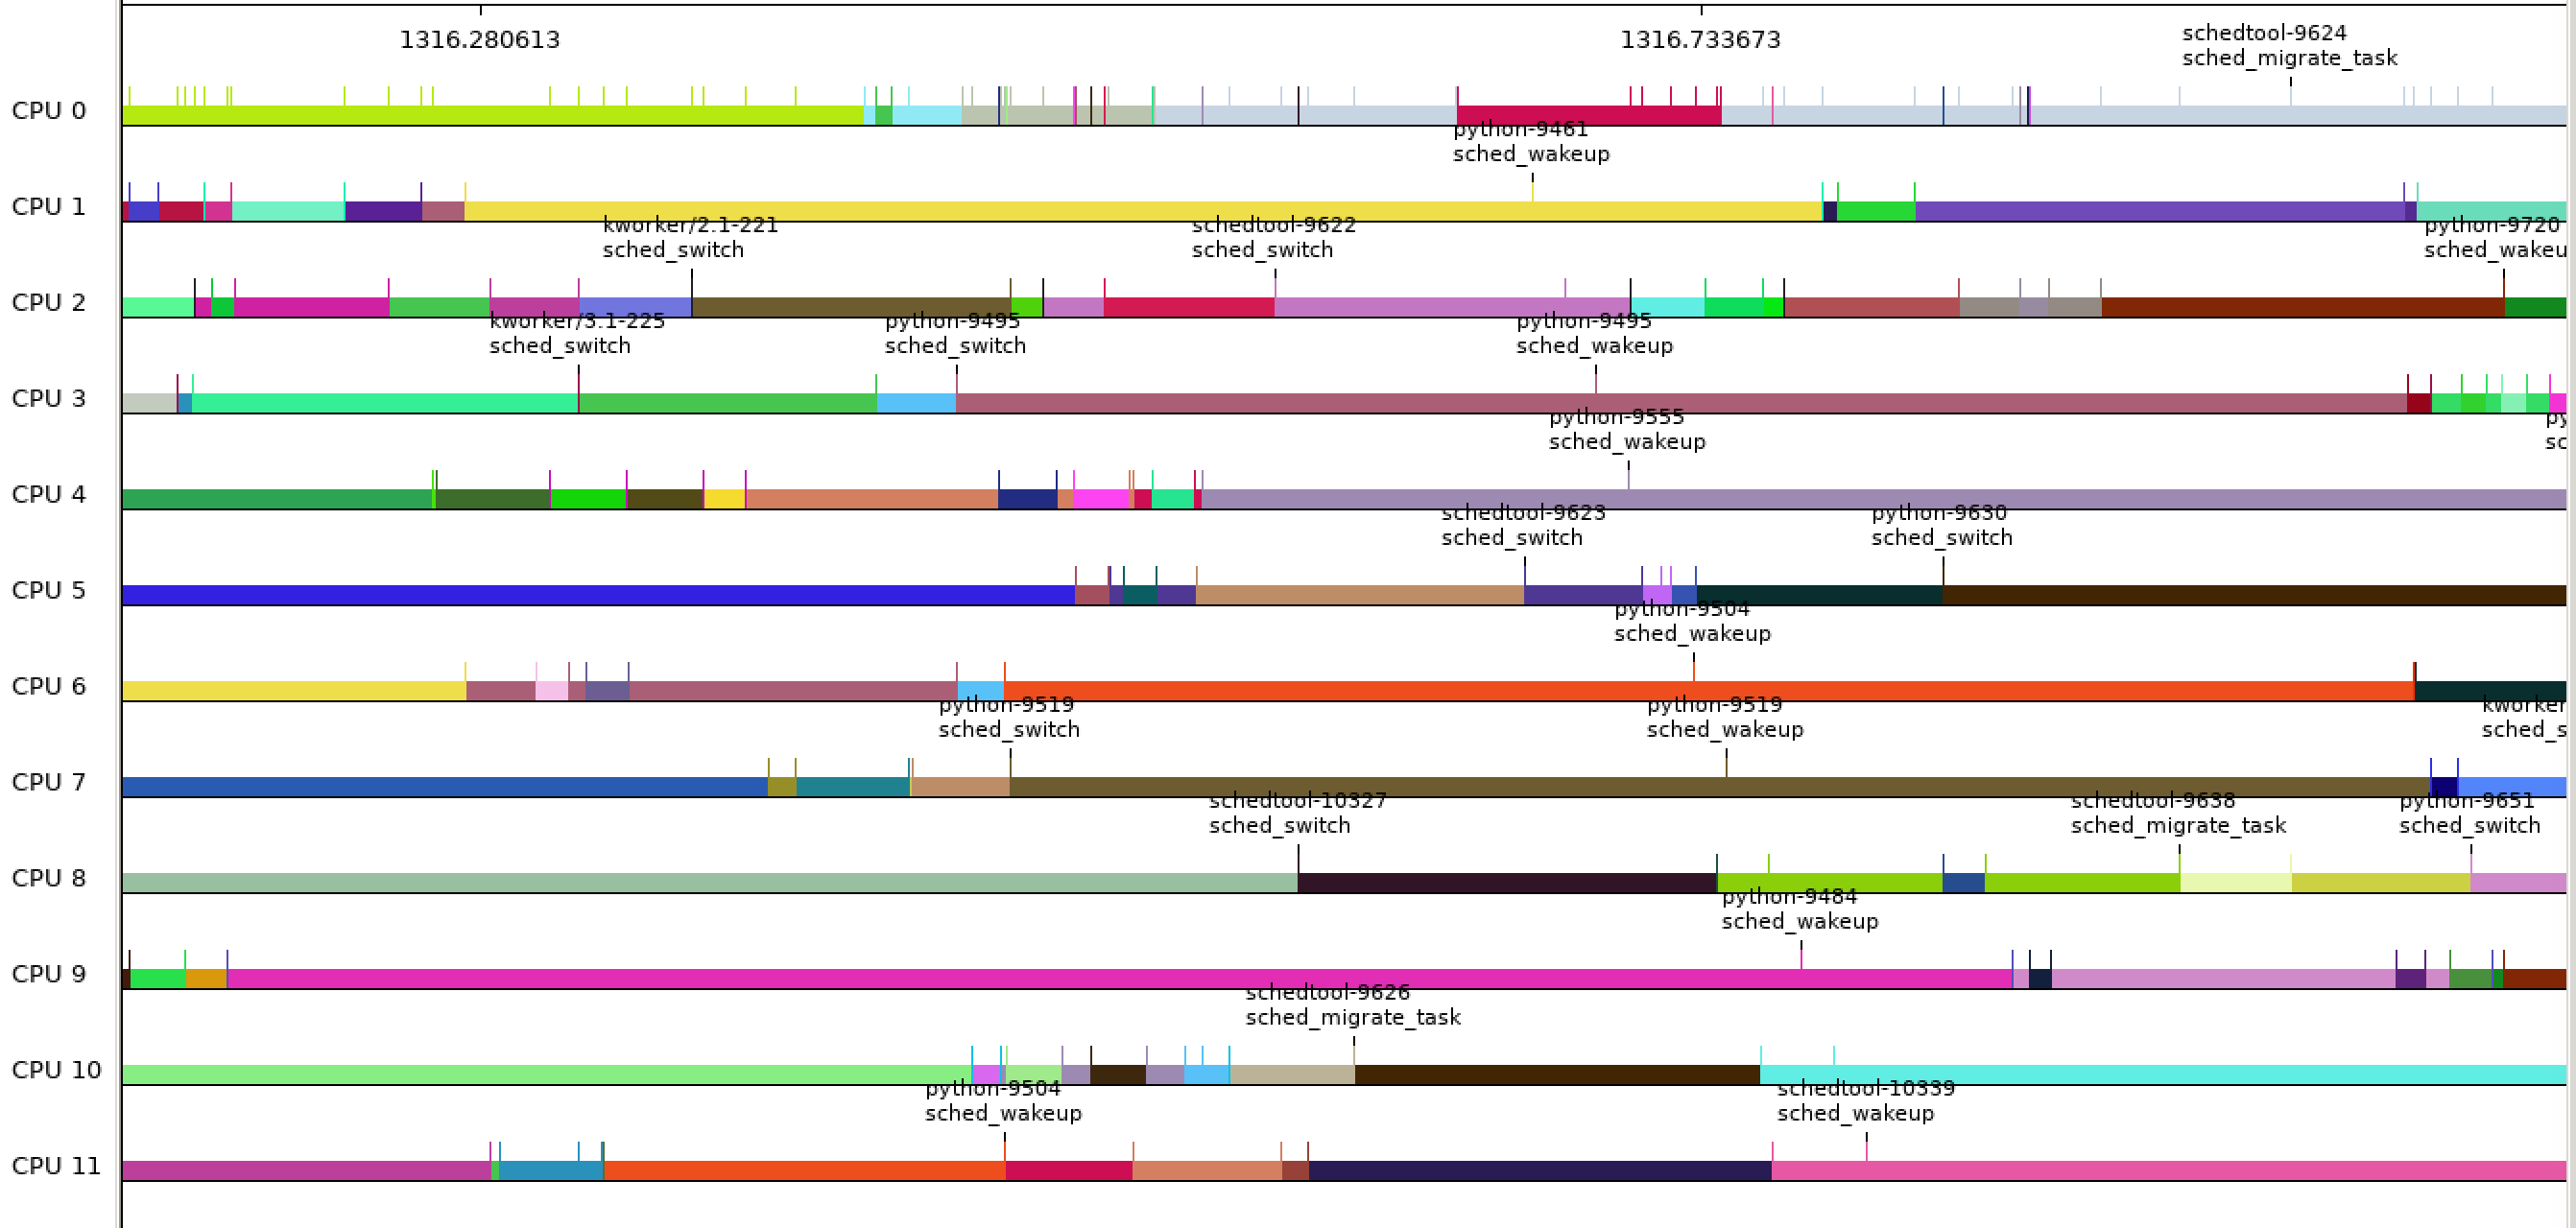}
\label{fig:kernel_sfs}
}
\vspace{-15pt}
\end{center}
\label{fig:kernelshark}
\caption{
The Gantt chart illustration of a 1-second scheduling period profiled by the {\small\texttt{trace-cmd}} tool~\cite{tracecmd} under Linux CFS (a) and {\proj} (b).  
Different function processes are marked in different colors. Note that colors may be reused across different functions. 
%functions' scheduling events profiled by Trace-Cmd tool. Fig  \ref{fig:kernel_cfs} plots gantt chart of CFS scheduler and Fig \ref{fig:kernel_sfs} plots gantt chart of proposed SFS scheduler. Both gantt charts includes about 1 second's profiled data. Functions are marked as different colors.
}
\vspace{-5pt}
\label{fig:kernelshark}
\end{figure}

\added{Figure~\ref{fig:kernel_cfs} shows an exemplar Gantt chart of CFS under multiple contending serverless functions: CFS frequently preempts function jobs (with changing colors), leading to longer aggregate waiting time with higher RTEs.}

%\vspace{-6pt}
\subsection{Uniform IAT}

In addition to the Poisson IAT distribution, we also tested a uniform IAT distribution; Figure~\ref{fig:random_IAT} shows a trend similar to the Poisson IAT configuration (\ref{fig:load_perf}). 
Results demonstrate that {\proj} plays a critical role in scheduling shorter functions smartly under relatively busier loads.

\begin{figure}[h]
%\vspace{-15pt}
\centering
\includegraphics[width=0.9\columnwidth]{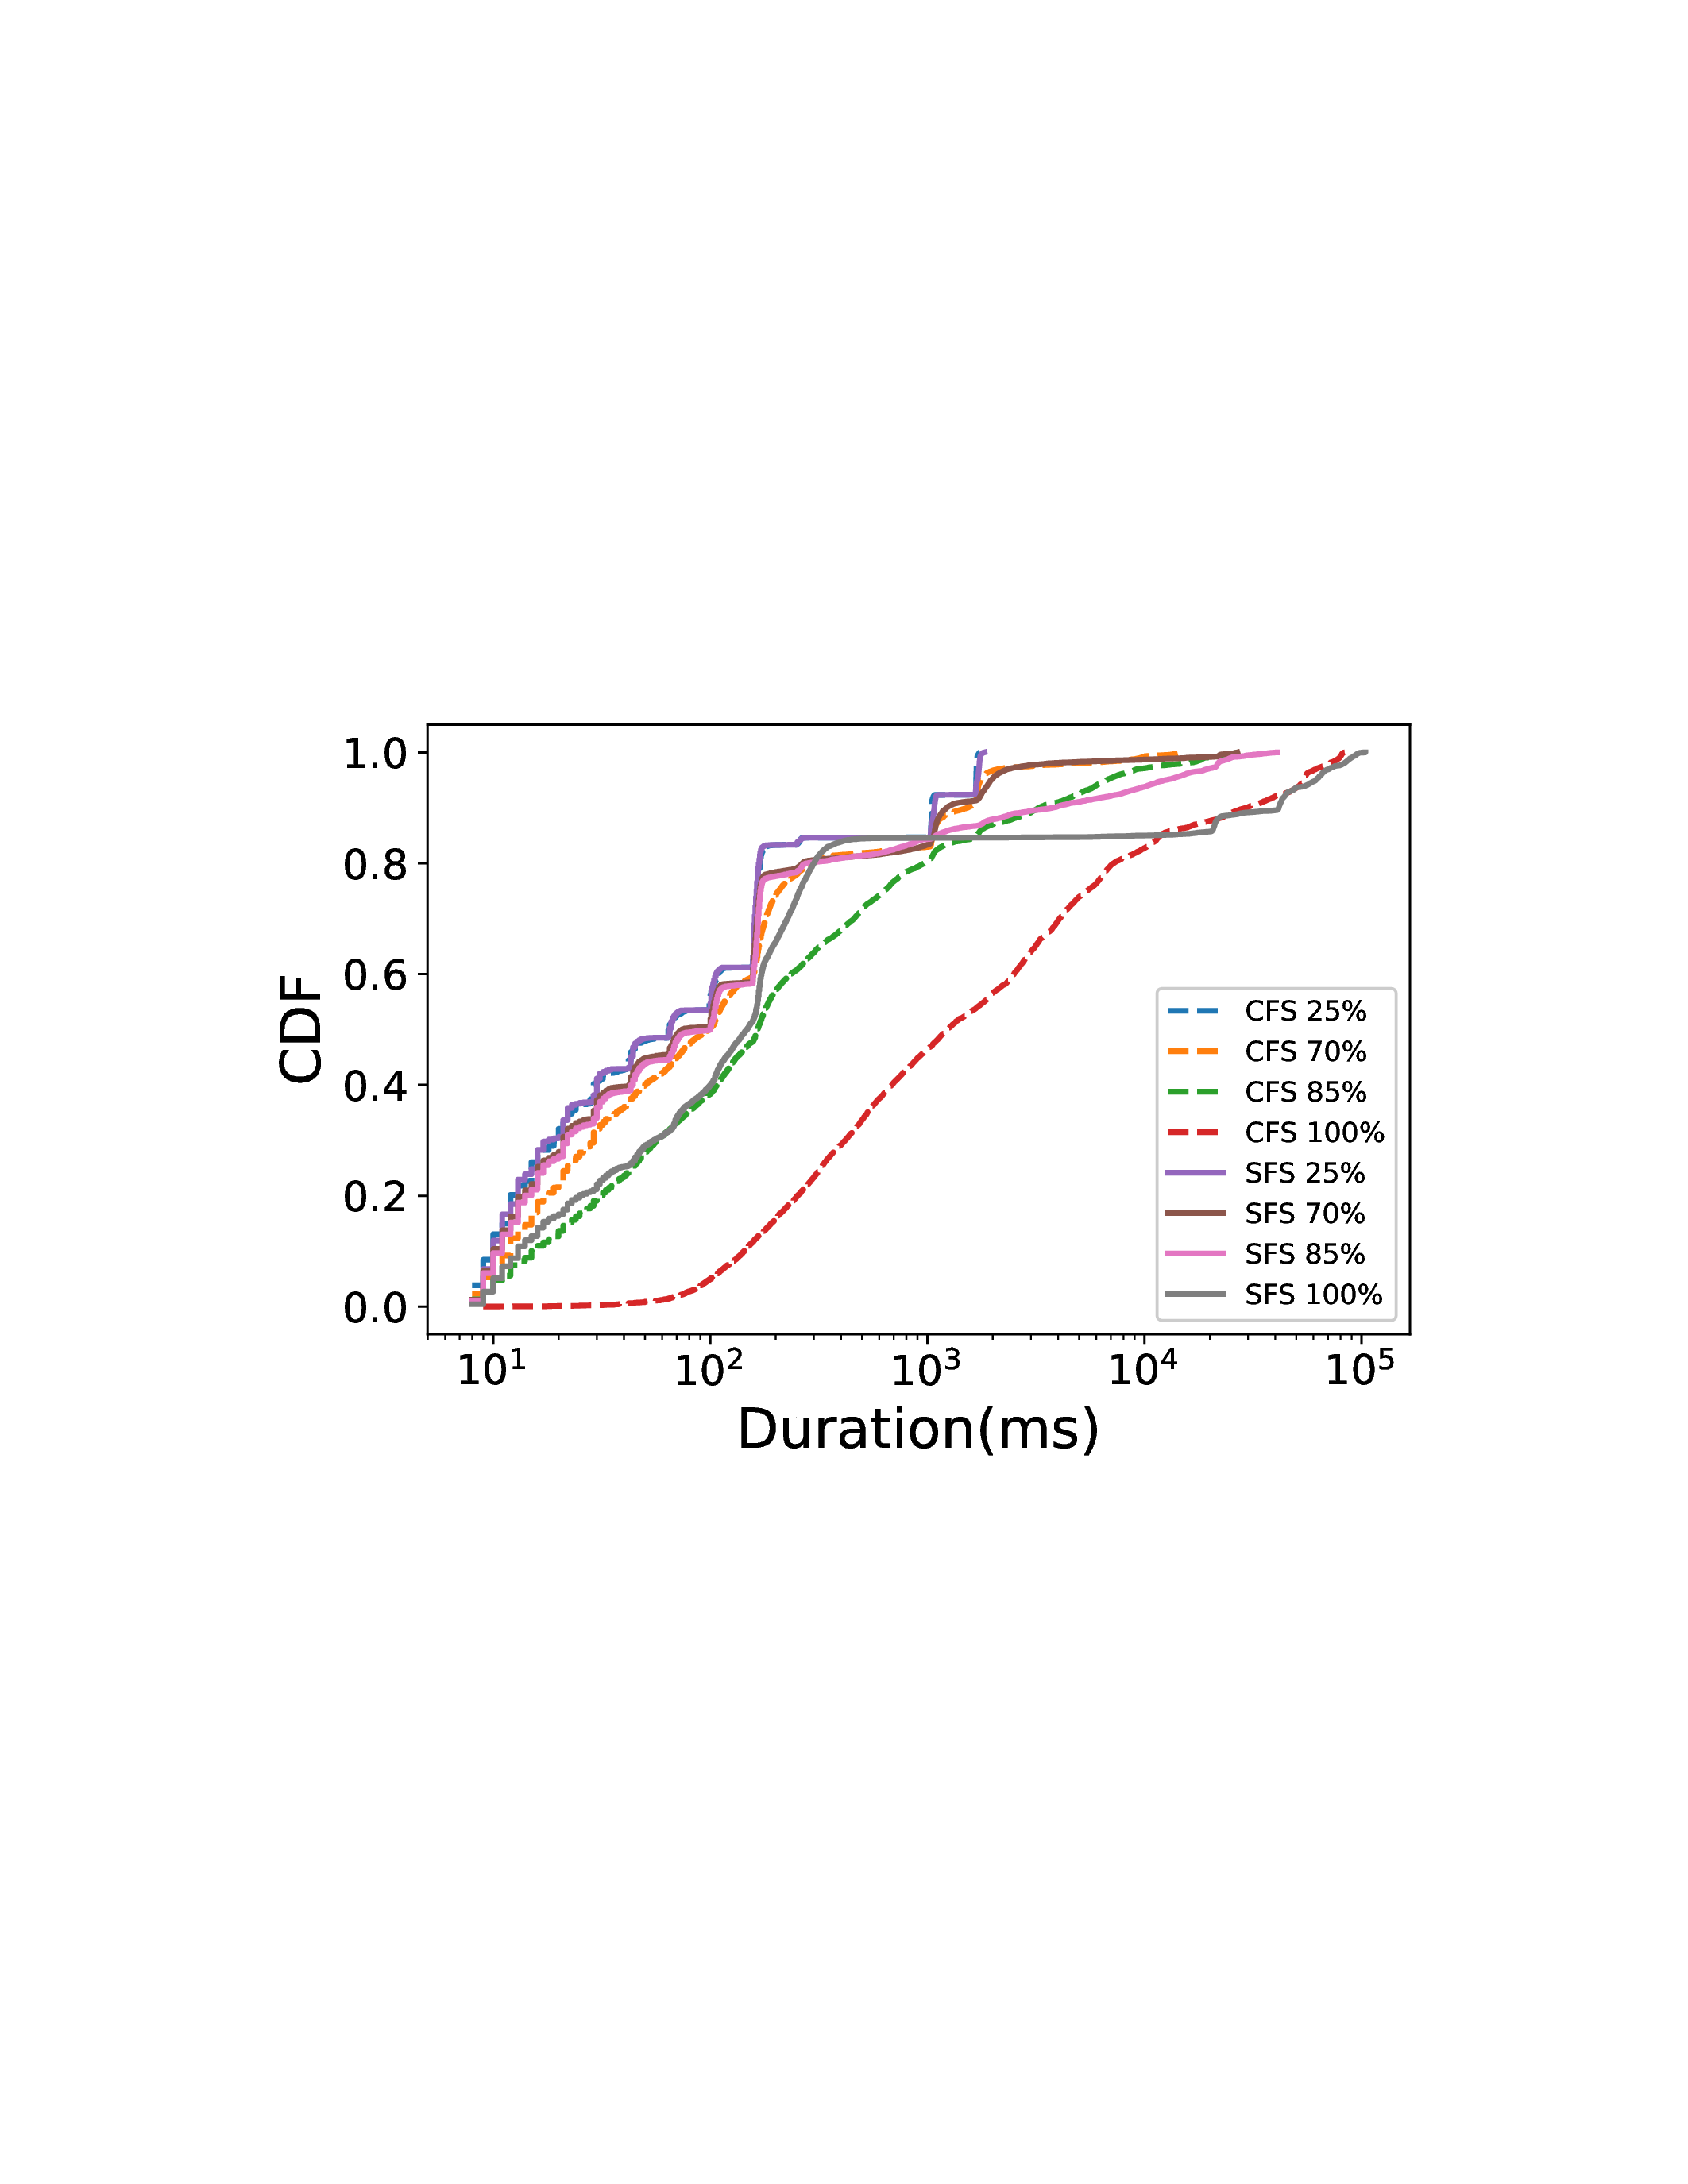}
\vspace{-5pt}
\caption{Performance under uniform IAT.
}
\vspace{-15pt}
\label{fig:random_IAT}
\end{figure}

%\subsection{Handling Starvation}
\subsection{Handling Long-Job Starvation}
\label{subsec:starvation} 

Starvation is an issue suffered by priority-based scheduling algorithms. {\proj} uses priority boosting~\cite{mlfq_solaris, mlfq_sigmetrics95}, which periodically move all jobs in the system to the topmost queue to mitigate this issue. 
%, by following Multi-level Feedback Queue(MLFQ) algorithm, 
%introduce boosting policy to mitigate this issue. 
%According to MLFQ logic, interactive jobs remains at topmost queues and long-term computation intensive task would fall to low priority queue, thus long-term task may have no chance on scheduling. MLFQ introduce "the priority boost" rule which periodically move all jobs in the system to the topmost queue.
The rule forces every task in the system having an opportunity to be scheduling.

We implemented priority boosting in {\proj}. After a configurable period of time $B$, {\proj} migrates a task from the CFS pool and reinserts it to the FILTER pool. 
{\proj} marks functions that have been boosted more than once and reduces the time slice $S$ for these functions to simulate the scheduling behavior of a proportional-share scheduler, say CFS.
%Boosting policy in SFS follow the same idea and SFS architecture makes boosting flexible and easily handled. After a fixed $T$ period time defined by users, SFS dequeue a task from CFS pool and resend it to the global. 
%Intuitively, SFS flag boosting jobs and fix time slice $S$ for these jobs as a small value to stimulate long-terms jobs behaving similar to Normal CFS jobs. We evaluate the efficacy of this strategy in \cref{subsec:sensitivity_analysis}.

\begin{figure}[h]
\begin{center}
\subfigure[Performance CDF.] {
\includegraphics[width=.45\textwidth]{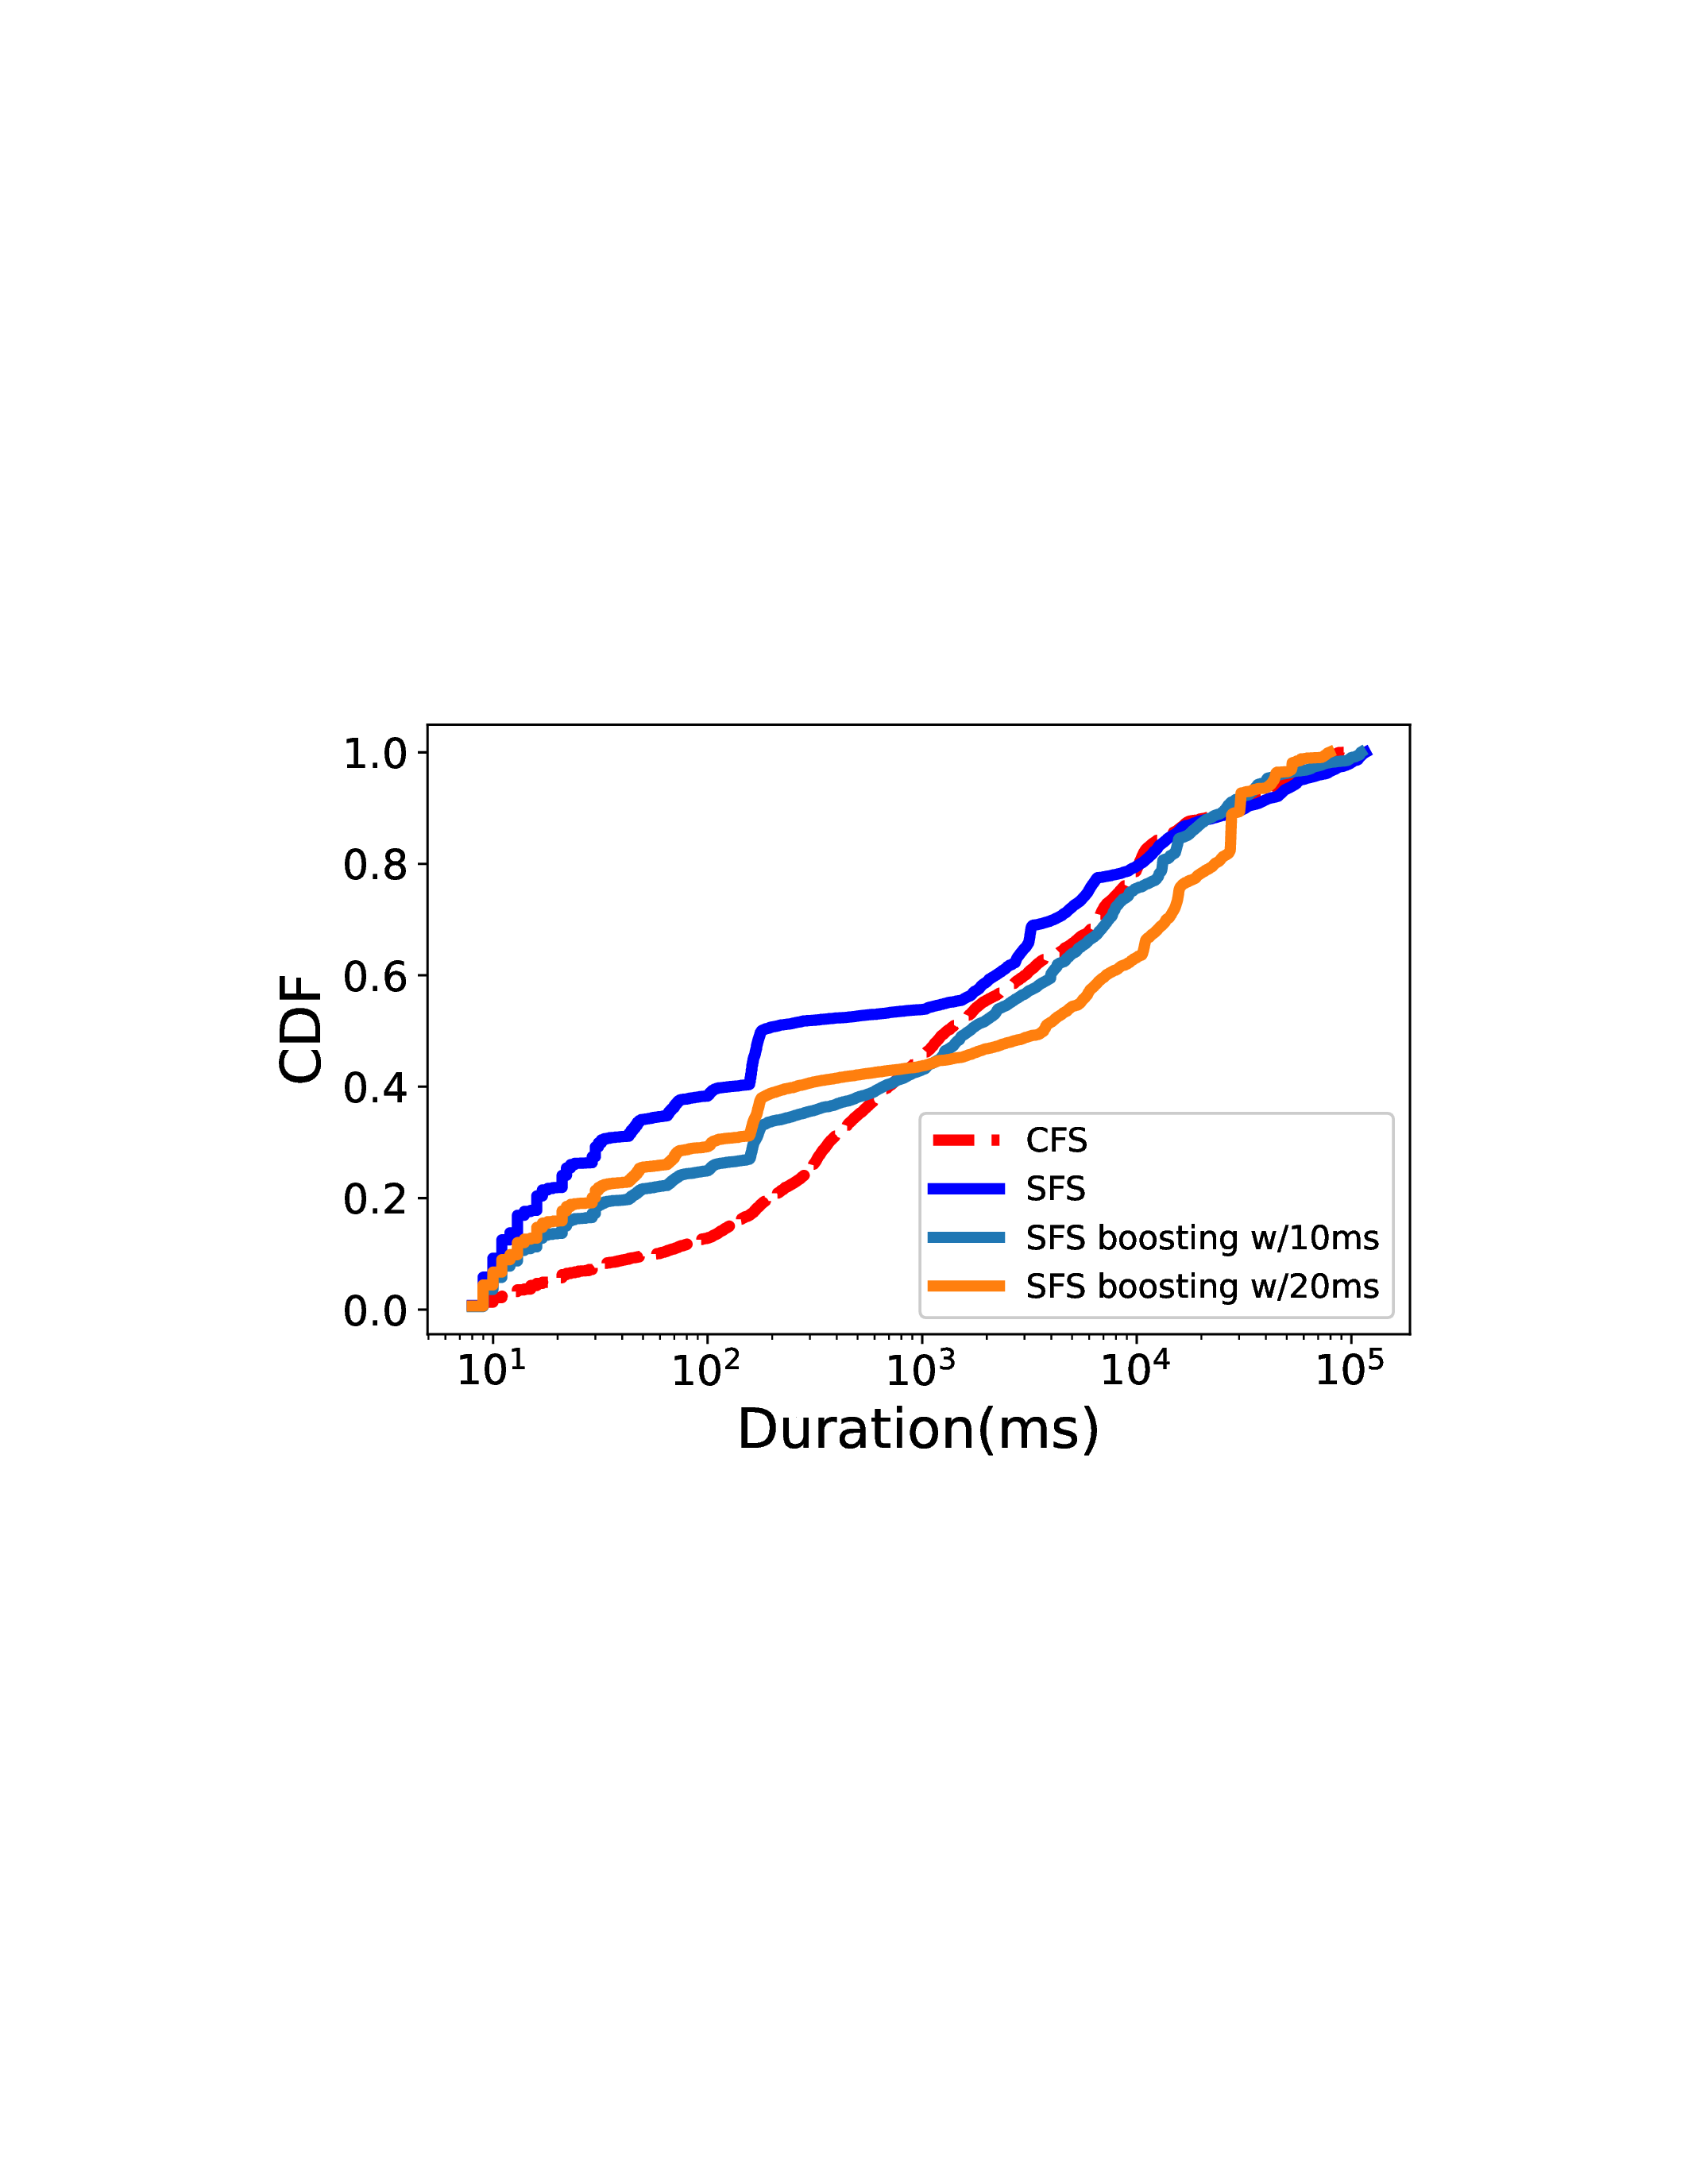}
\label{fig:starvation_whole}
}
\hspace{-12pt}
\subfigure[CDF of the top 10 percent longest jobs.] {
\includegraphics[width=.45\textwidth]{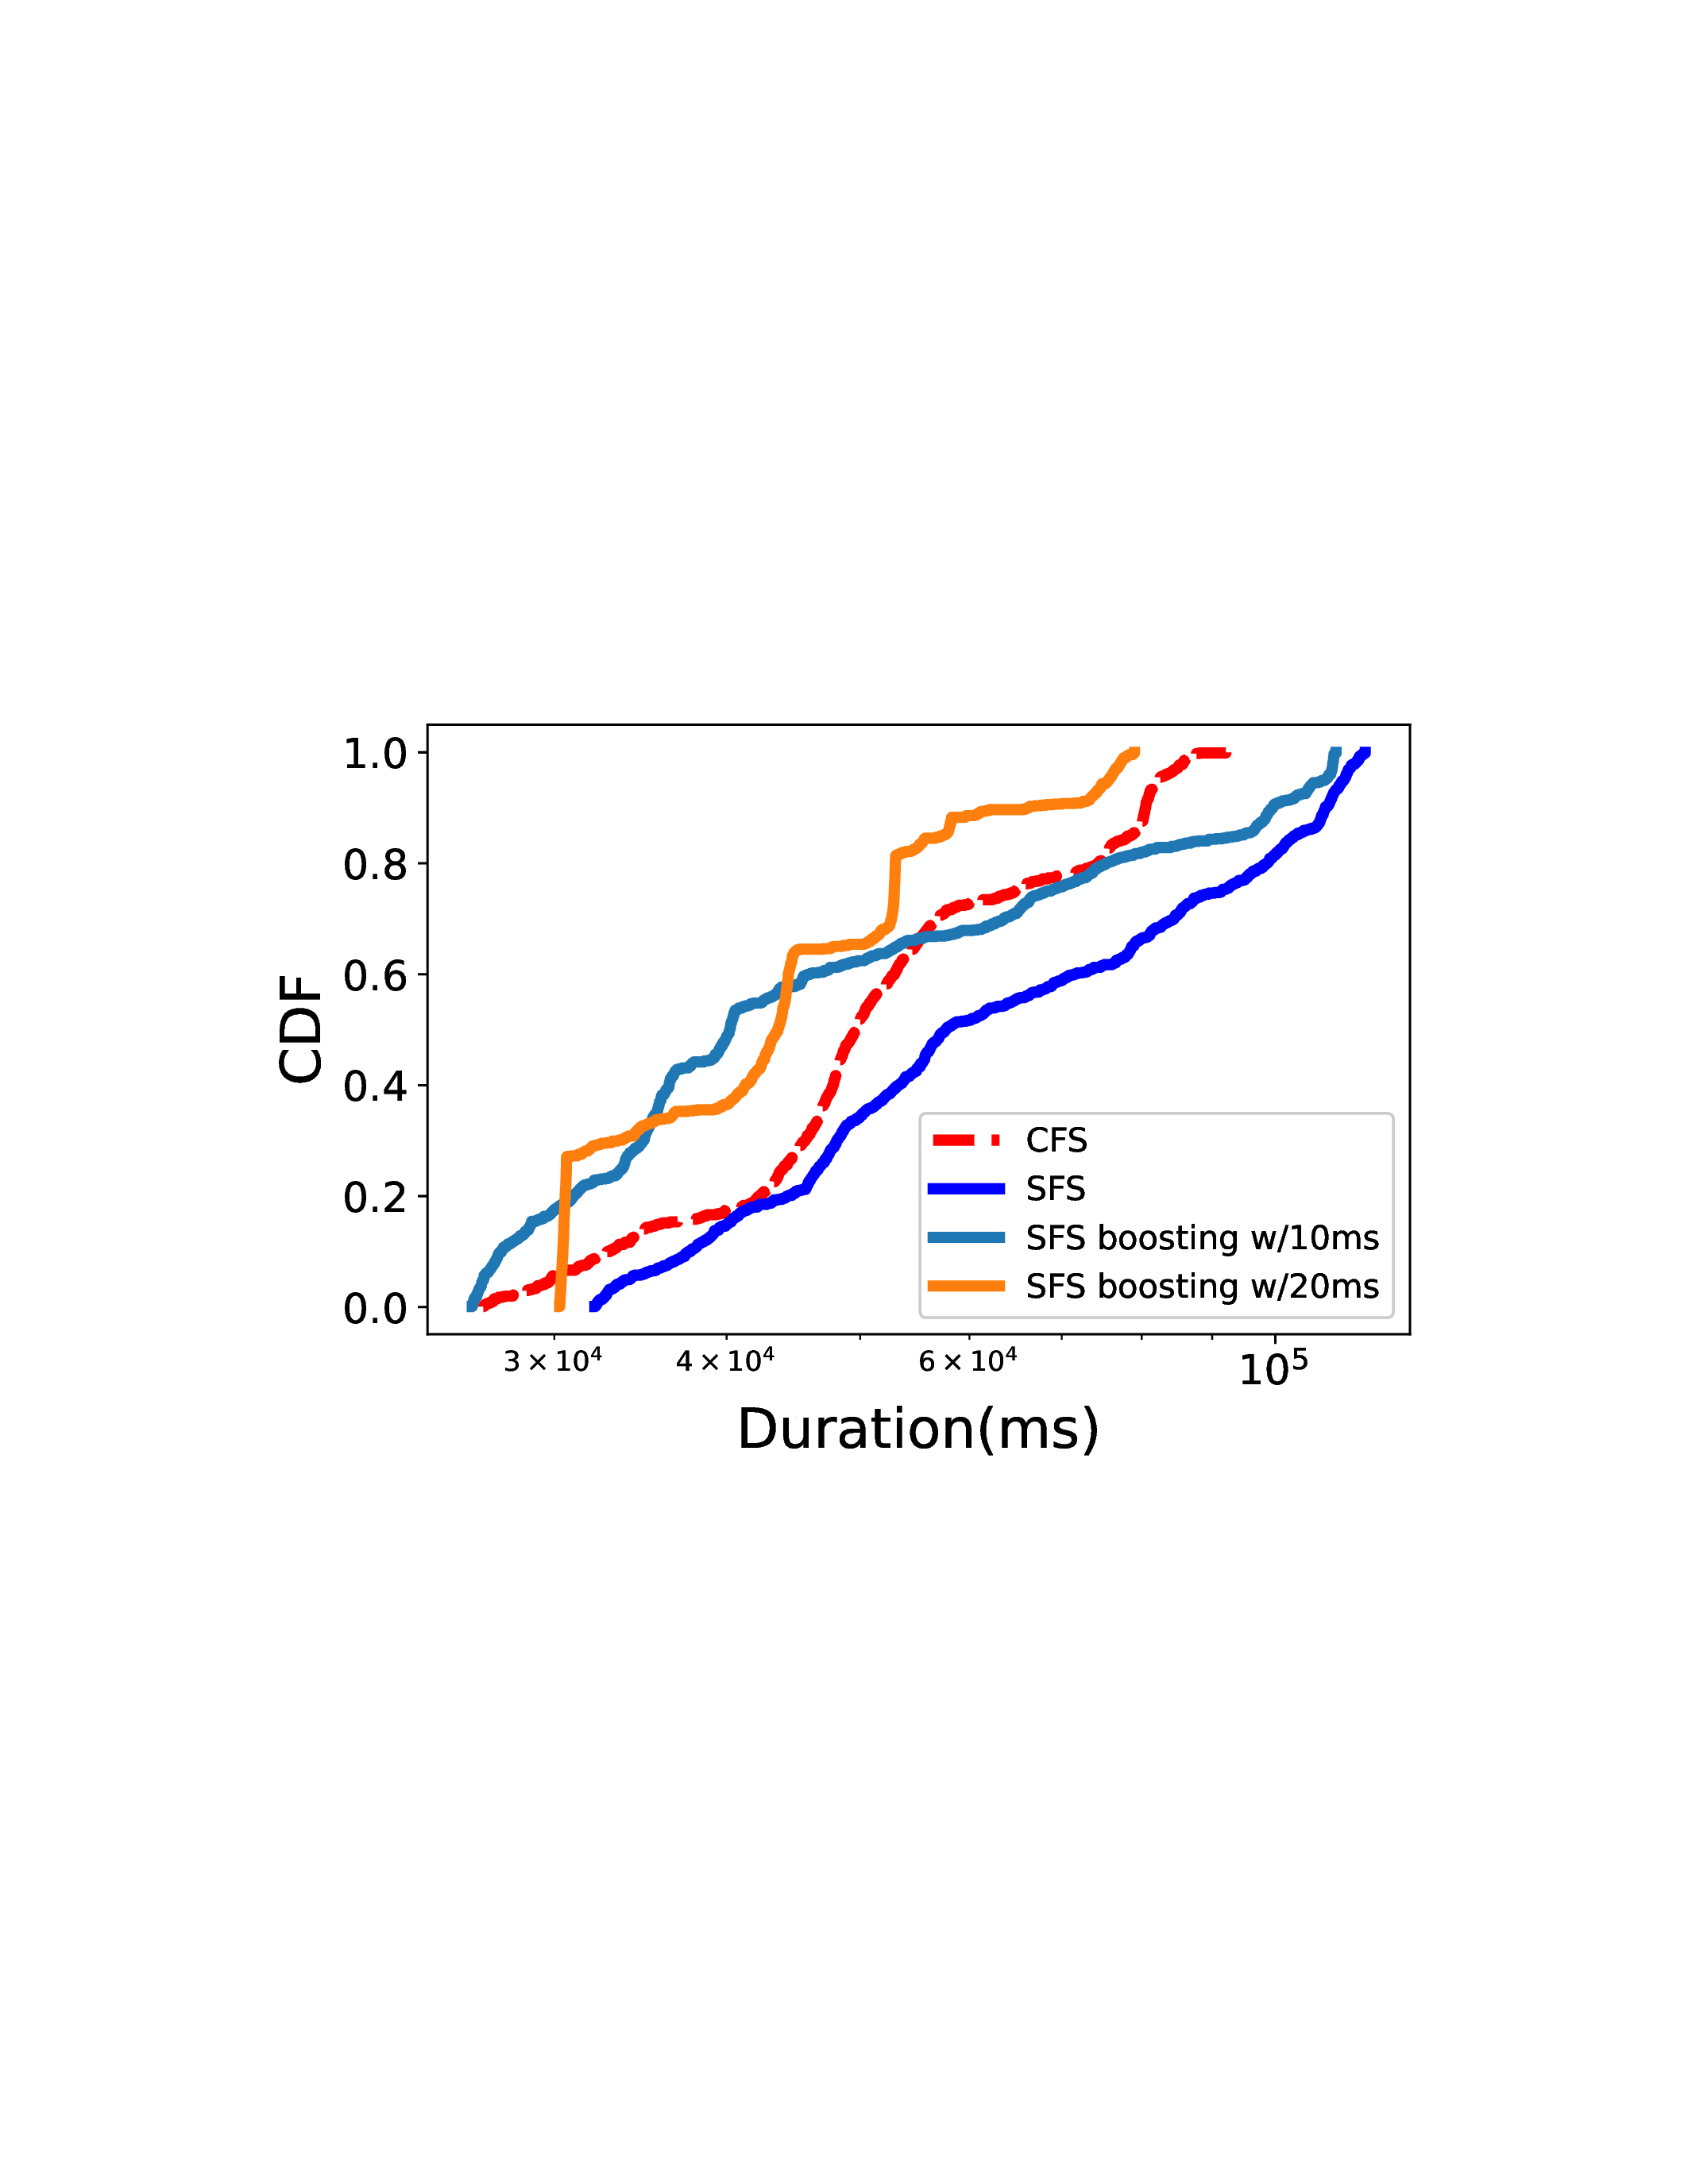}
\label{fig:starvation_long}
}
%\hspace{-12pt}
%\subfigure[CDF of function's memory configuration.] {
%\includegraphics[width=.23\textwidth]{plots/function_memory.pdf}
%\label{fig:function_memory}
%}
\vspace{-5pt}
\caption{
Effectiveness of priority boosting.
%{\proj}'s a
%Performance of boosting 
%parameters with 50~ms, 100~ms, and 200~ms. 
}
\label{fig:starvation}
\end{center}
\vspace{-10pt}
\end{figure}

%To evaluate our priority boosting policy, we 
We evaluated the priority boosting policy with two picked boosting period, 10~ms, and 20~ms. As shown in Figure~\ref{fig:starvation}(b), priority boosting effectively reduced the execution duration of long functions, leading to much improved tail latency than {\proj} without the priority boosting enabled. The improved performance for the top $10\%$ longest functions does not come for free: as shown in Figure~\ref{fig:starvation}(a), priority boosting affects the performance of relatively shorter functions. The boosting period $B$ needs to be carefully tuned in order to strike a balance between short functions and long functions. 

%\added{\noindent\textbf{Handling Starvation.}To evaluate performance of boosting policy, we set boost period as $10$ms and $20$ms respectively. As shown in Fig\ref{fig:starvation}(b), boosting offers more scheduling opportunities to long-term tasks so that SFS can achieve a better performance in tail latency. However, boosting sacrifies overall performance according to Fig\ref{fig:starvation}(a). Frequency of boosting need to carefully defined which controls trade-off between overall performance and starvation.}

\begin{figure*}[h]
\vspace{-5pt}
\begin{center}
\subfigure[Azure-sampled.] {
\includegraphics[width=.23\textwidth]{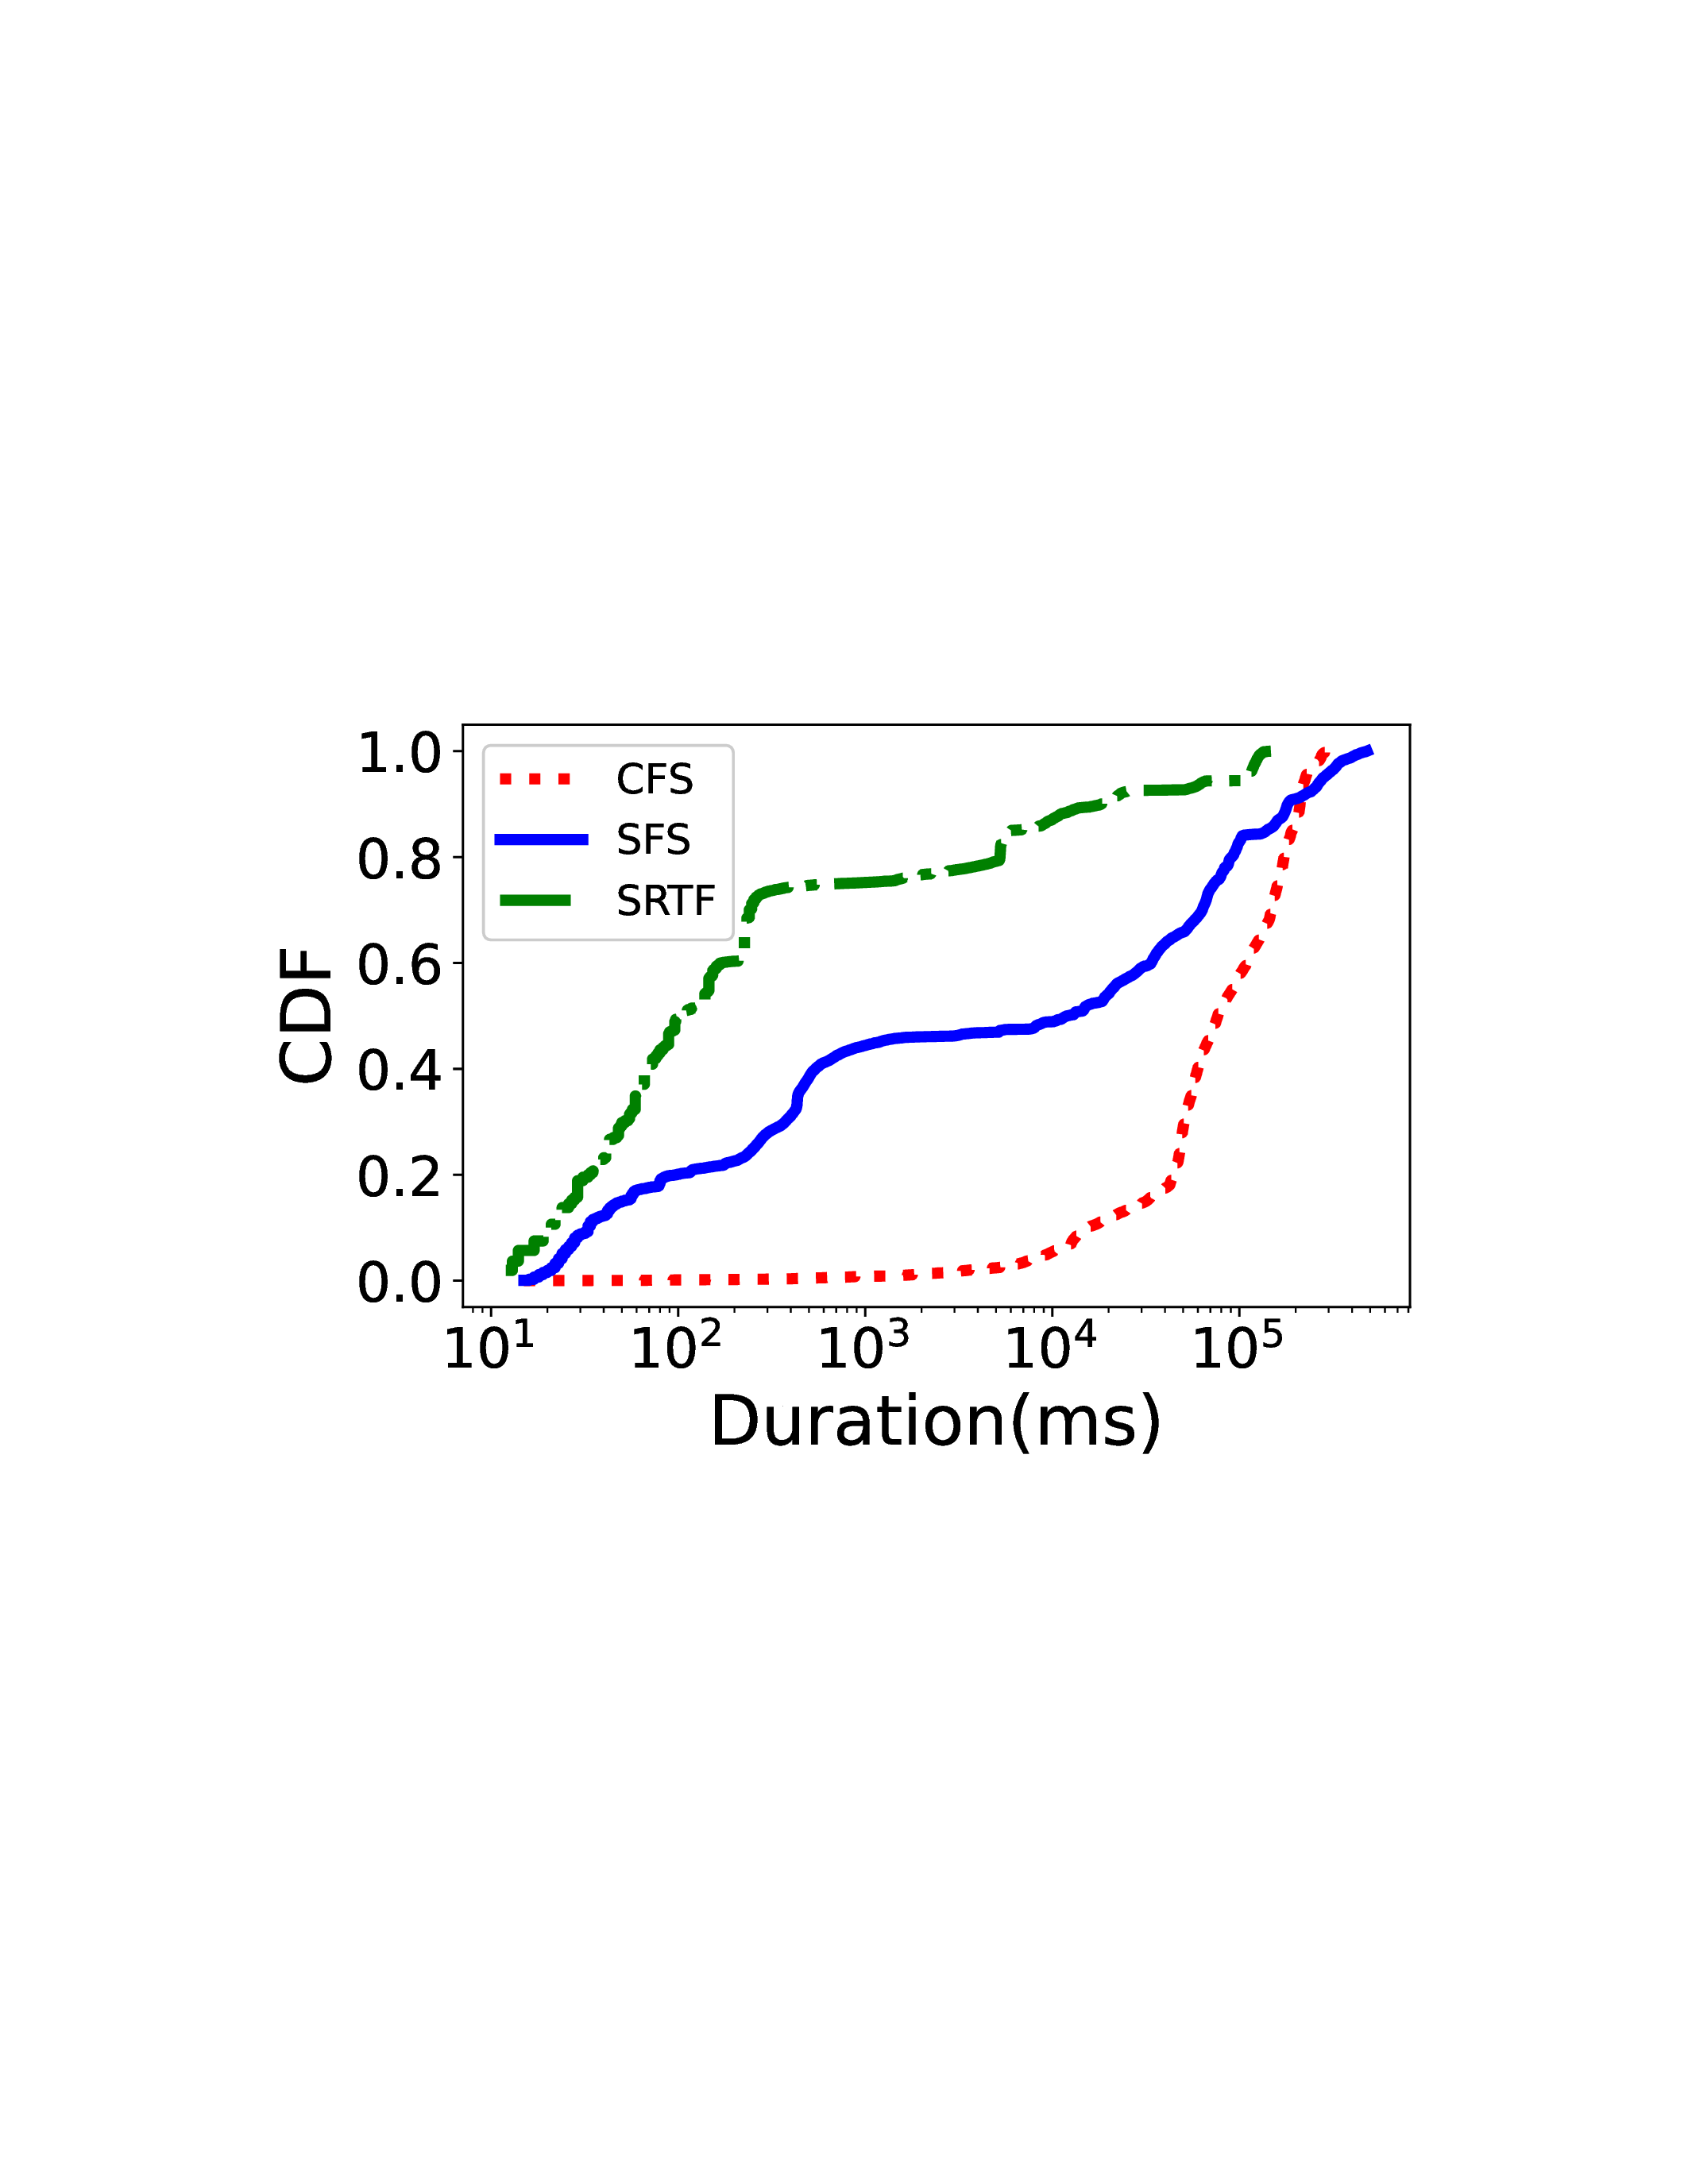}
\label{fig:azure_cdf}
}
\hspace{-9pt}
%\vspace{-20pt}
\subfigure[Short-dominant.] {
\includegraphics[width=.23\textwidth]{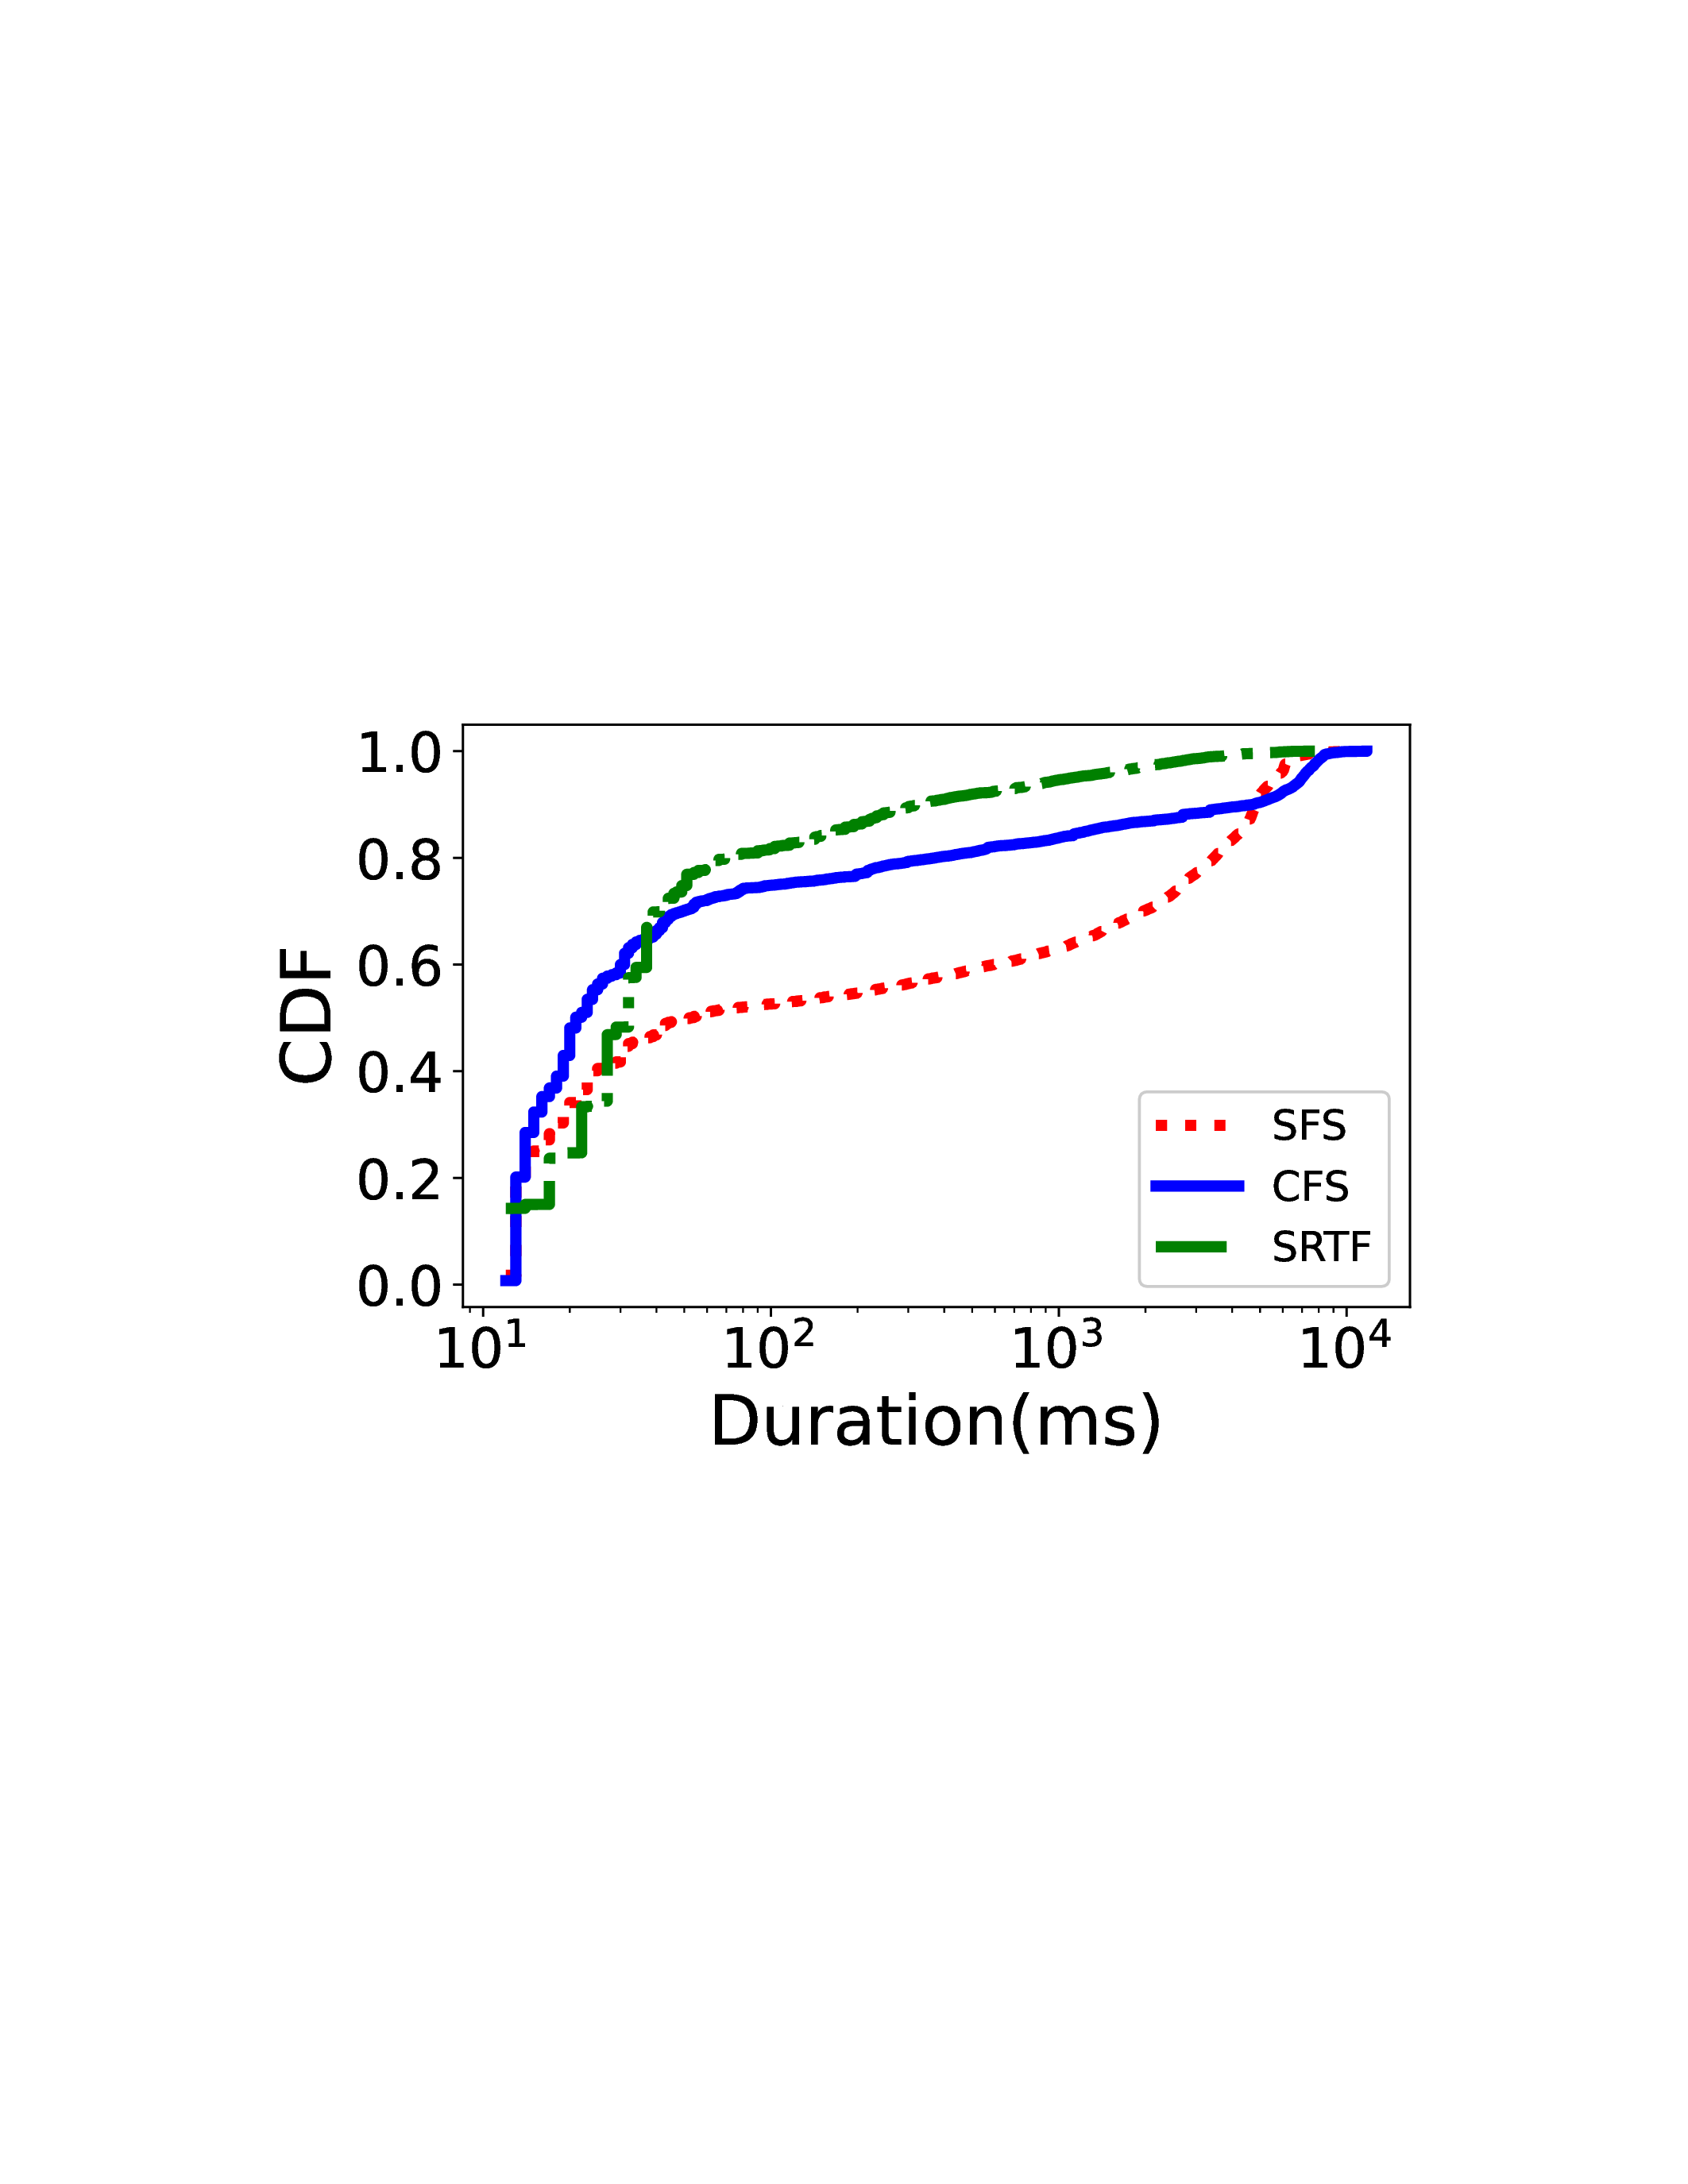}
\label{fig:short_cdf}
}
\hspace{-9pt}
\subfigure[Long-dominant.] {
\includegraphics[width=.23\textwidth]{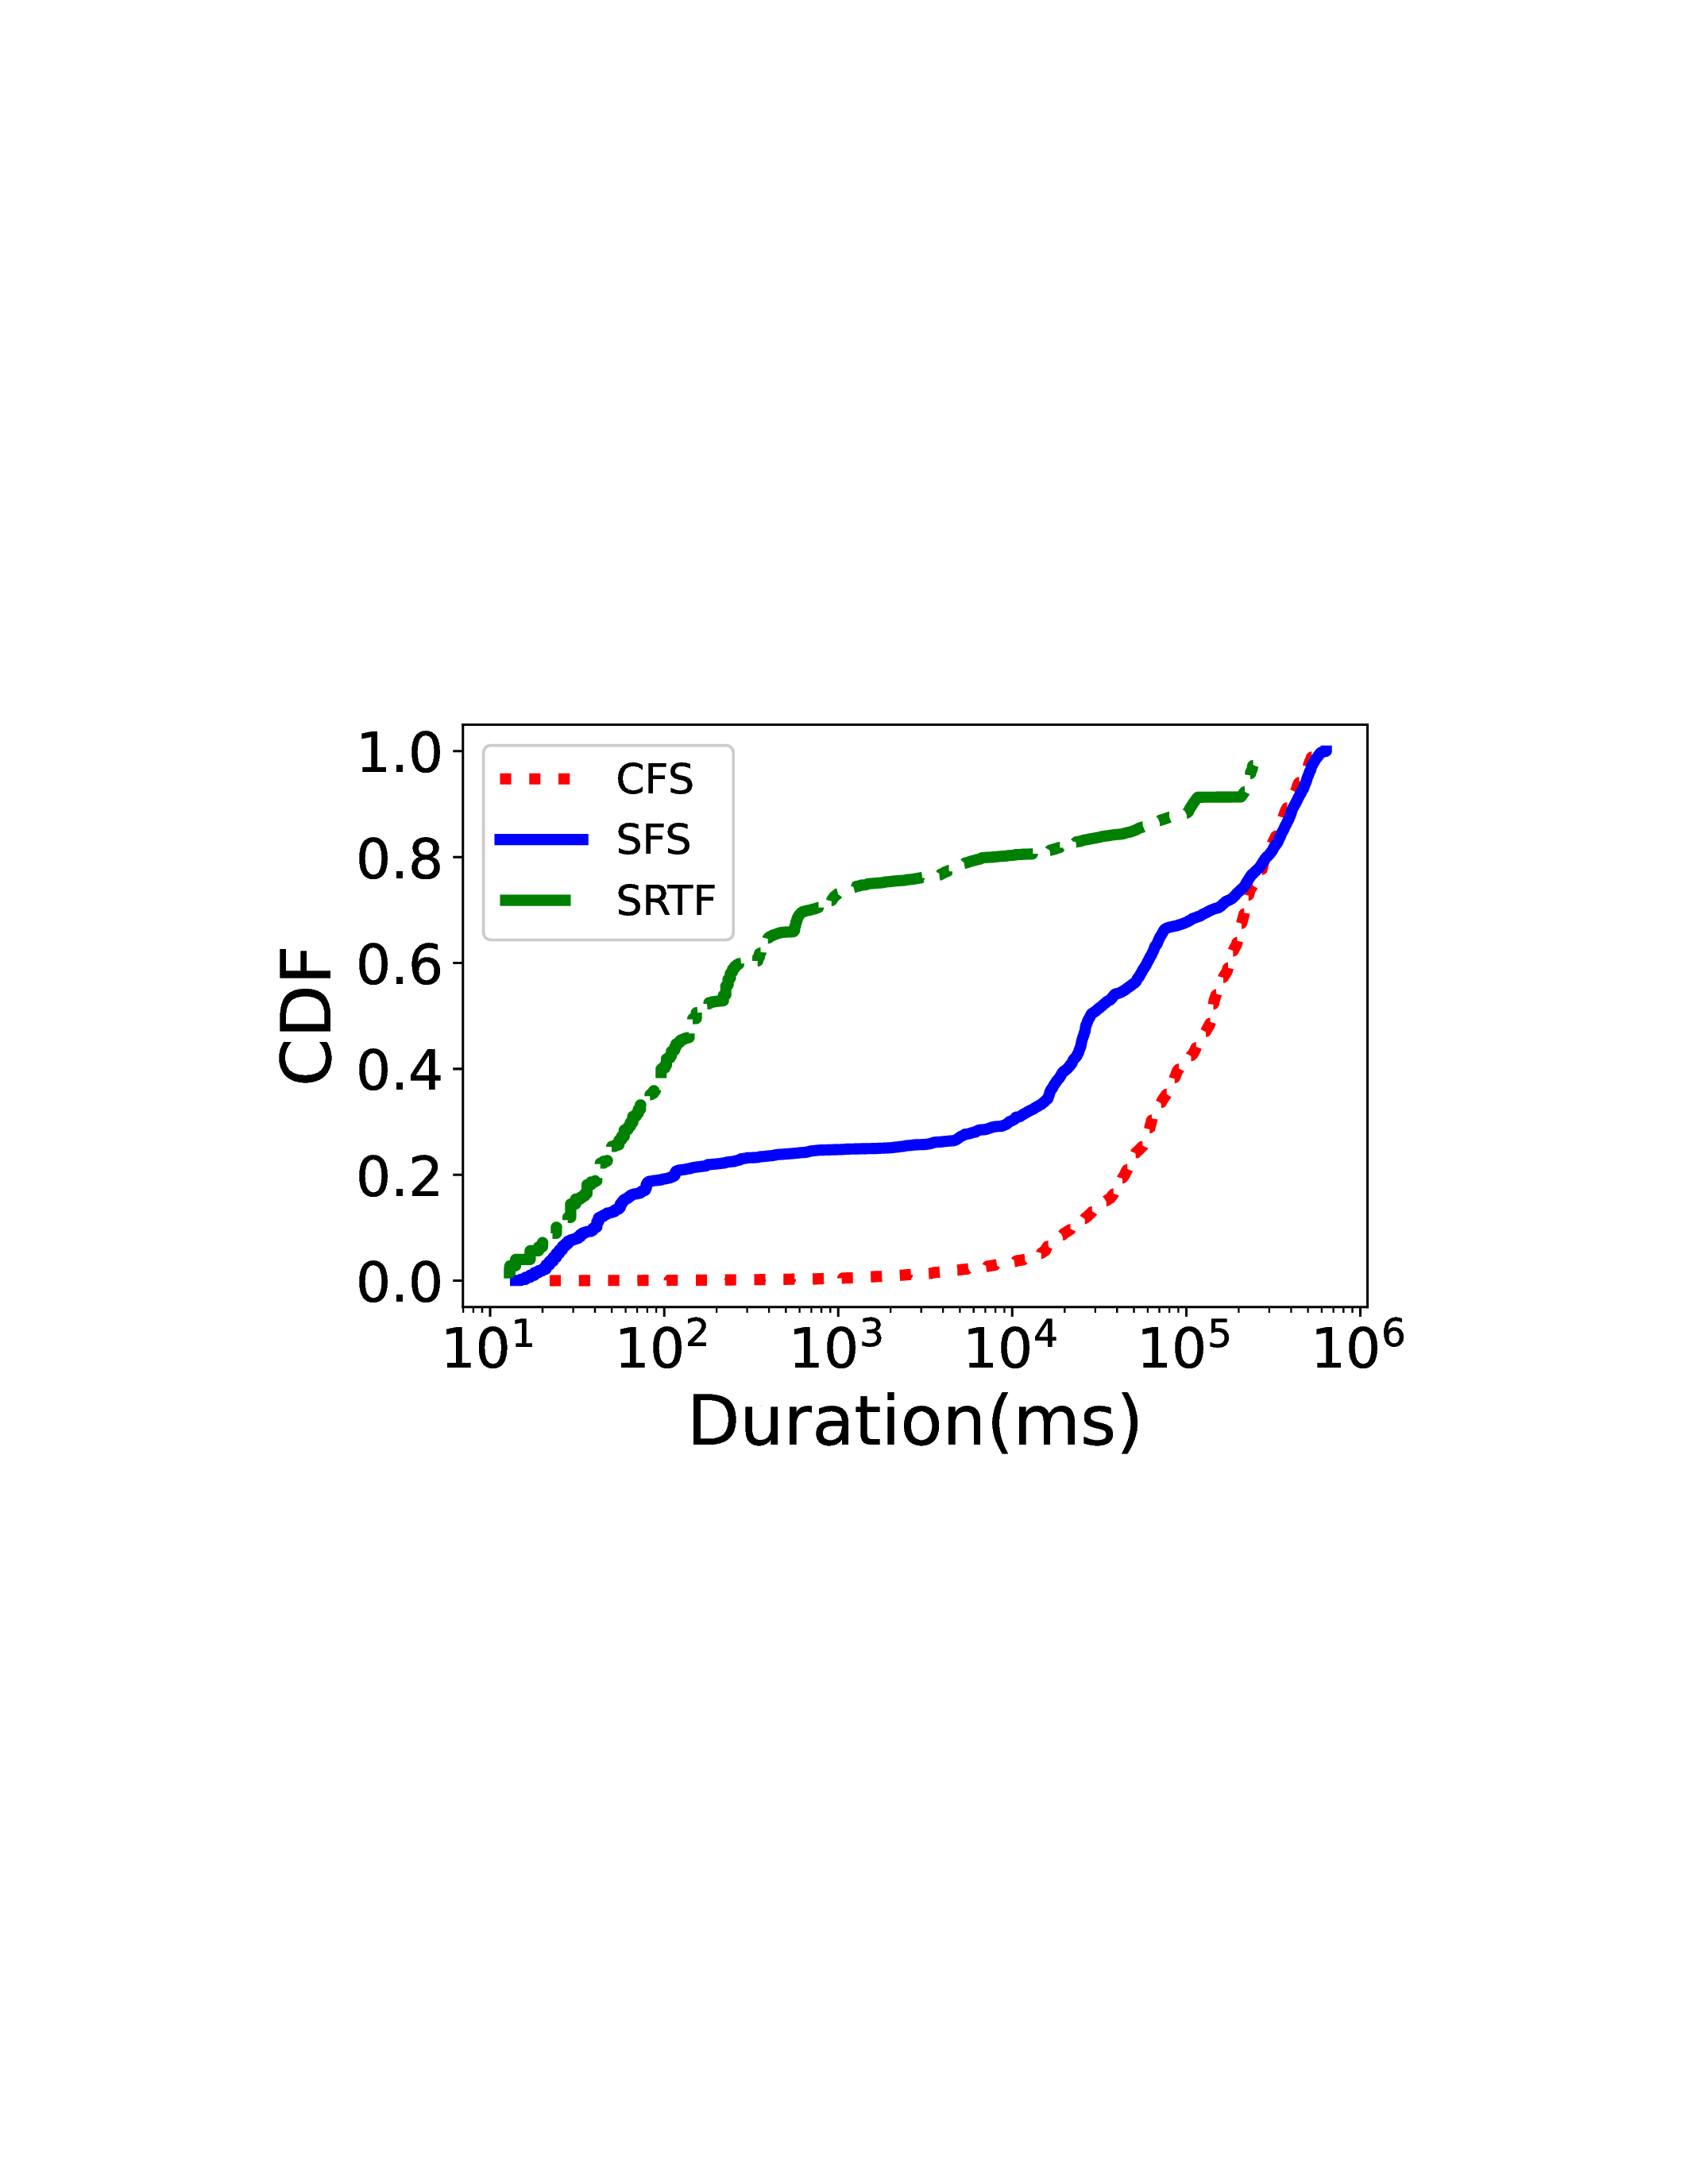}
\label{fig:long_cdf}
}
\hspace{-9pt}
\subfigure[Uniform.] {
\includegraphics[width=.23\textwidth]{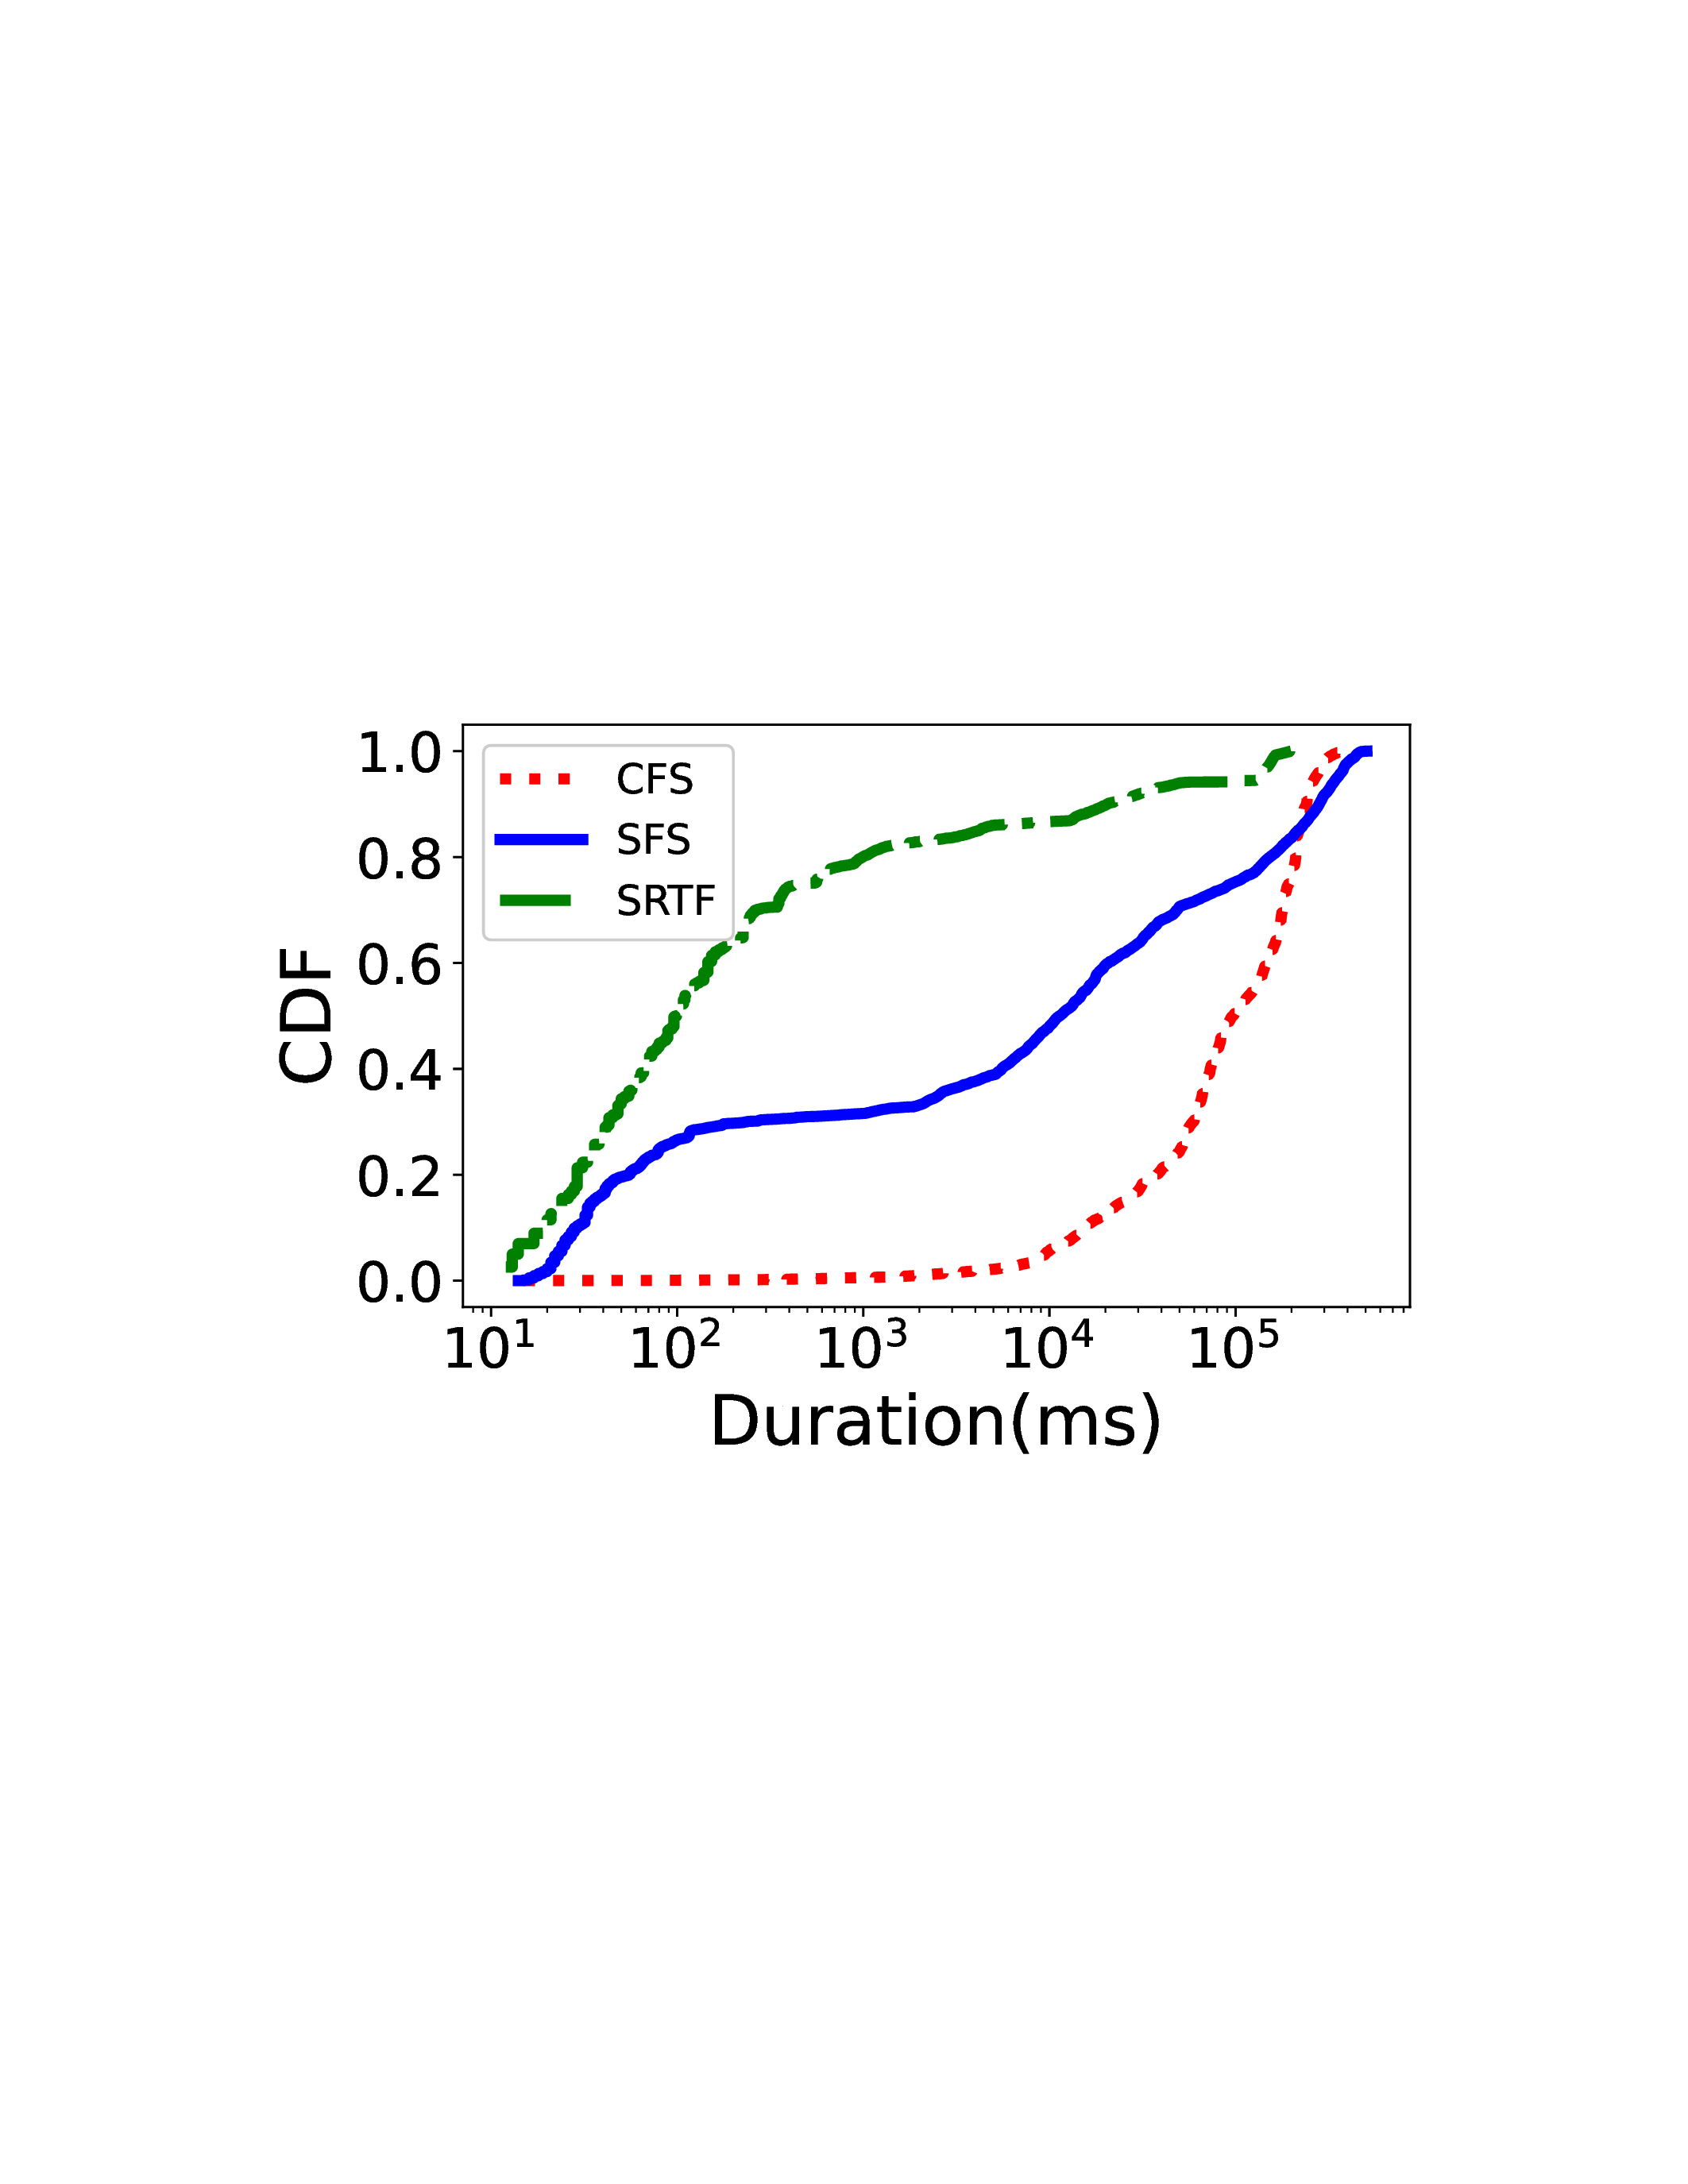}
\label{fig:unif_cdf}
}
%\hspace{-9pt}
\subfigure[Azure-sampled.] {
\includegraphics[width=.23\textwidth]{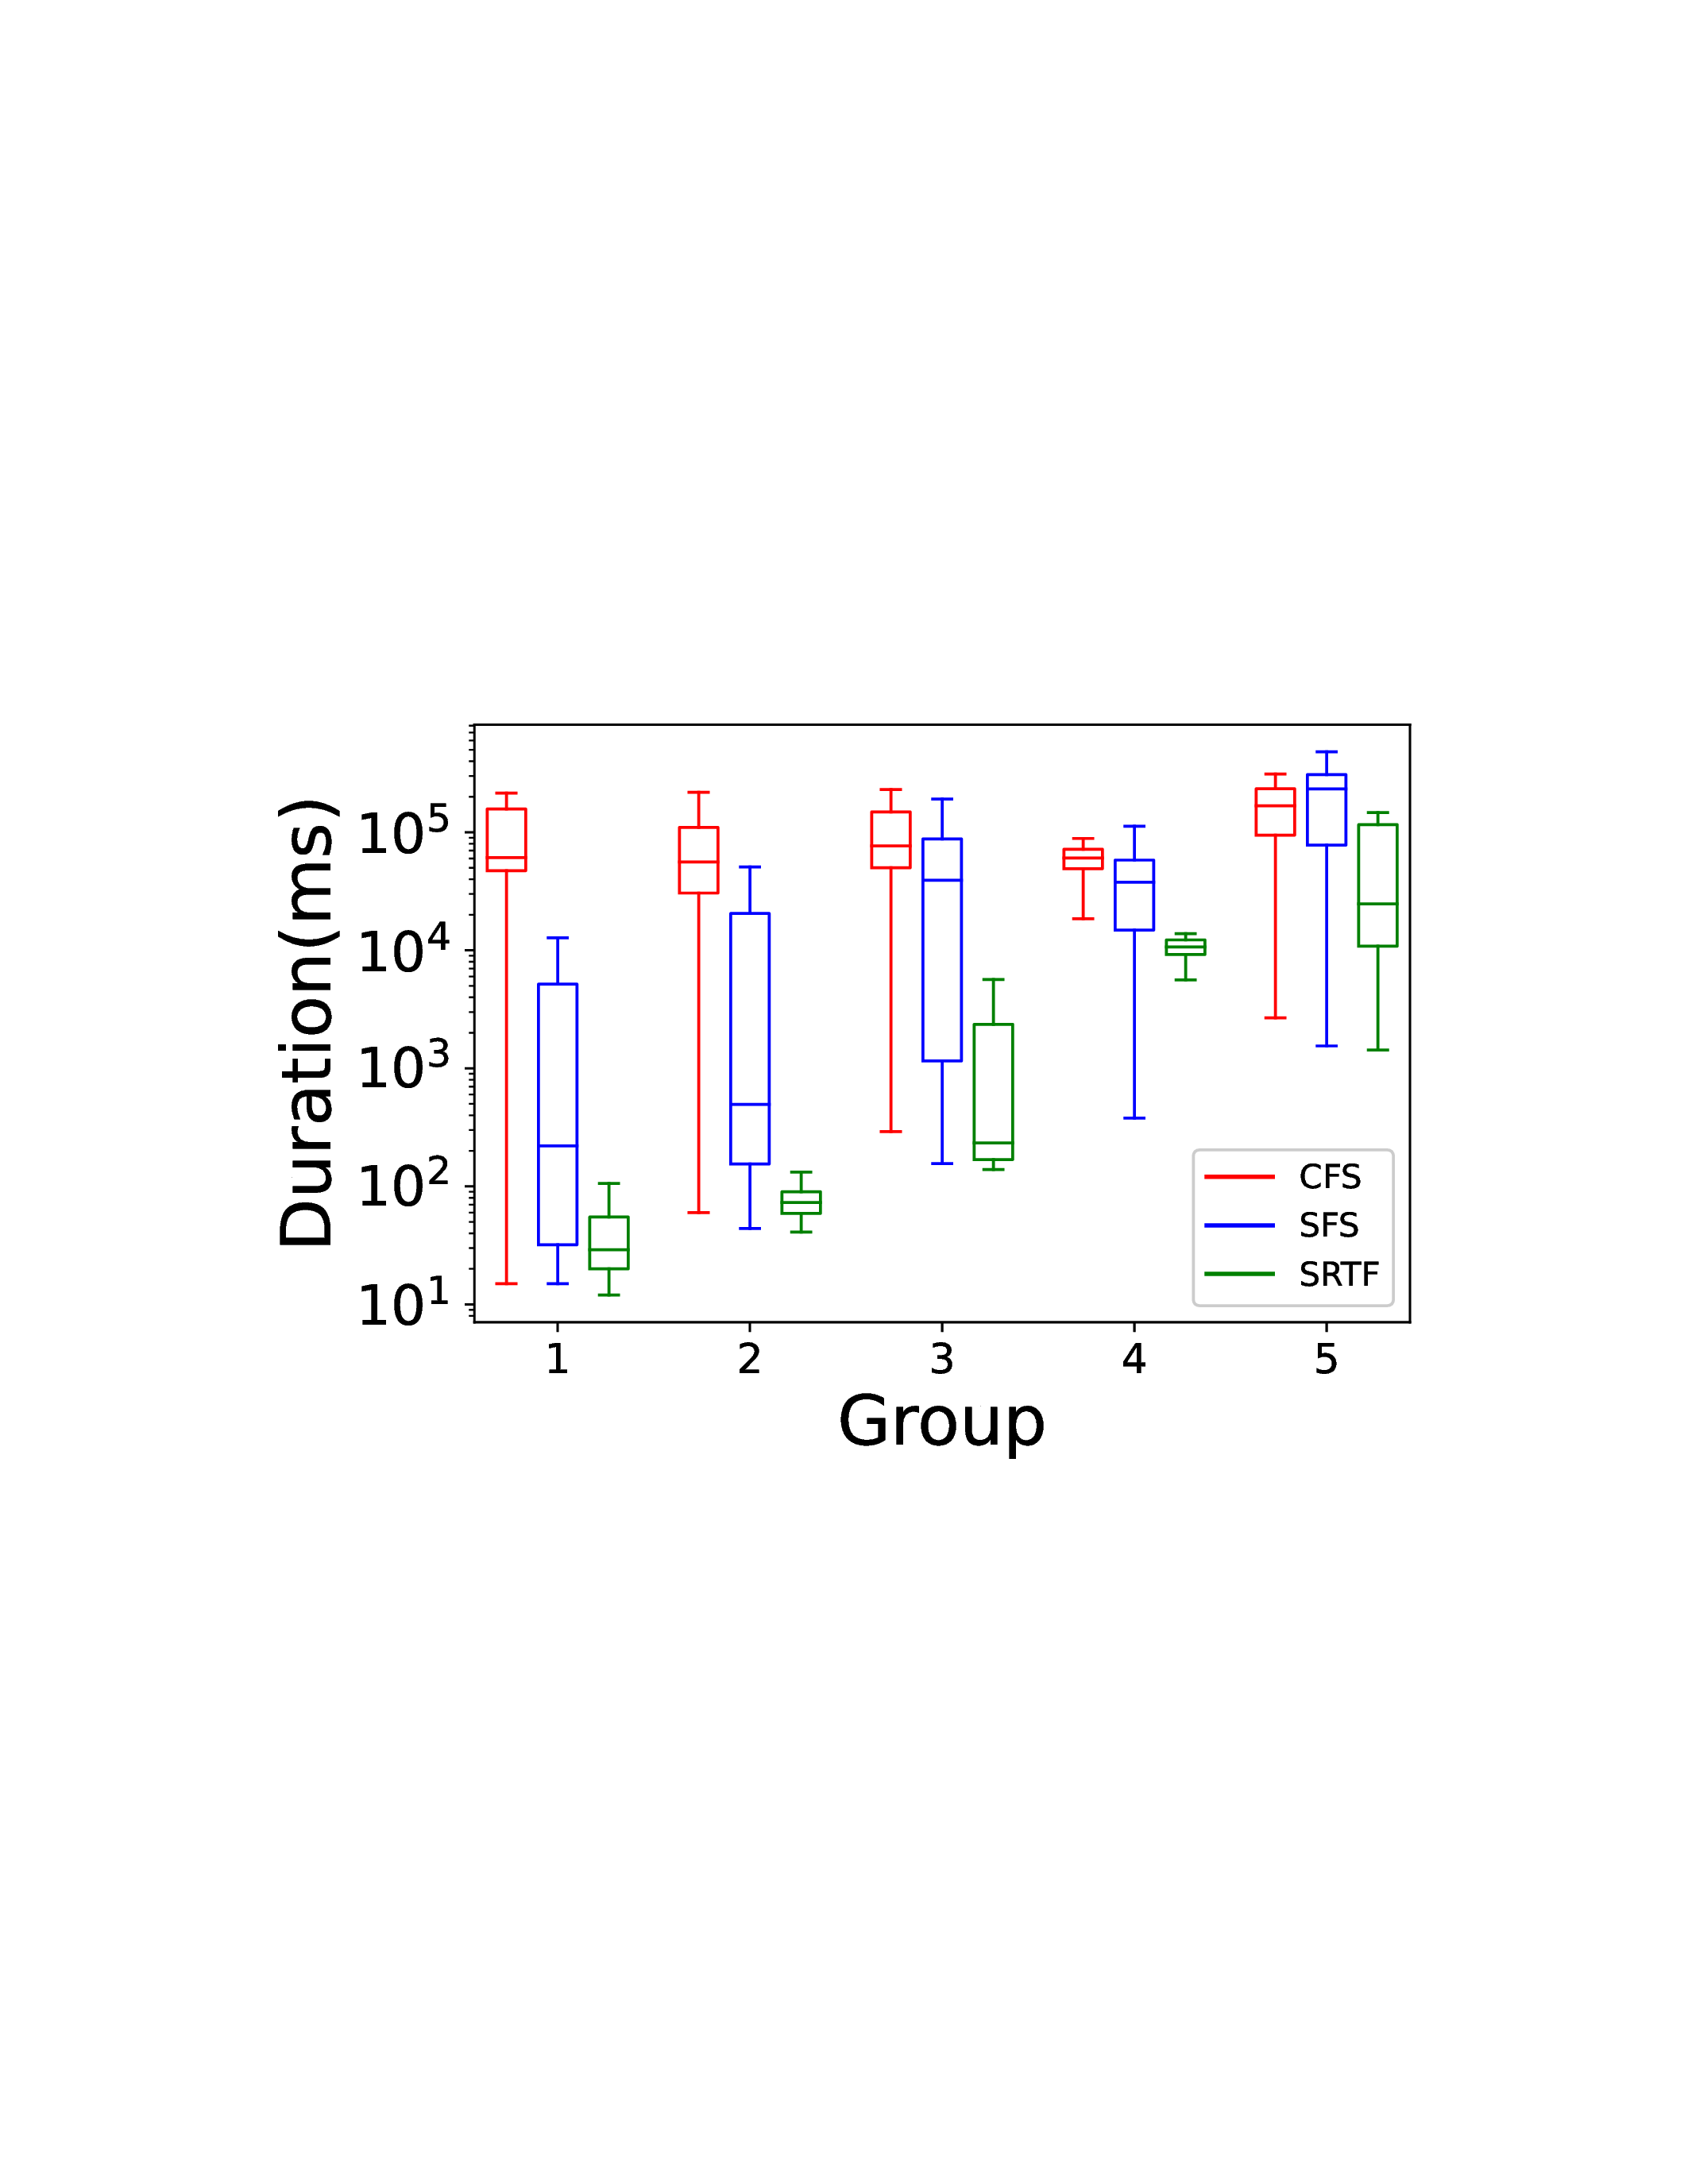}
\label{fig:azure_box}
}
\hspace{-9pt}
\subfigure[Short-dominant.] {
\includegraphics[width=.23\textwidth]{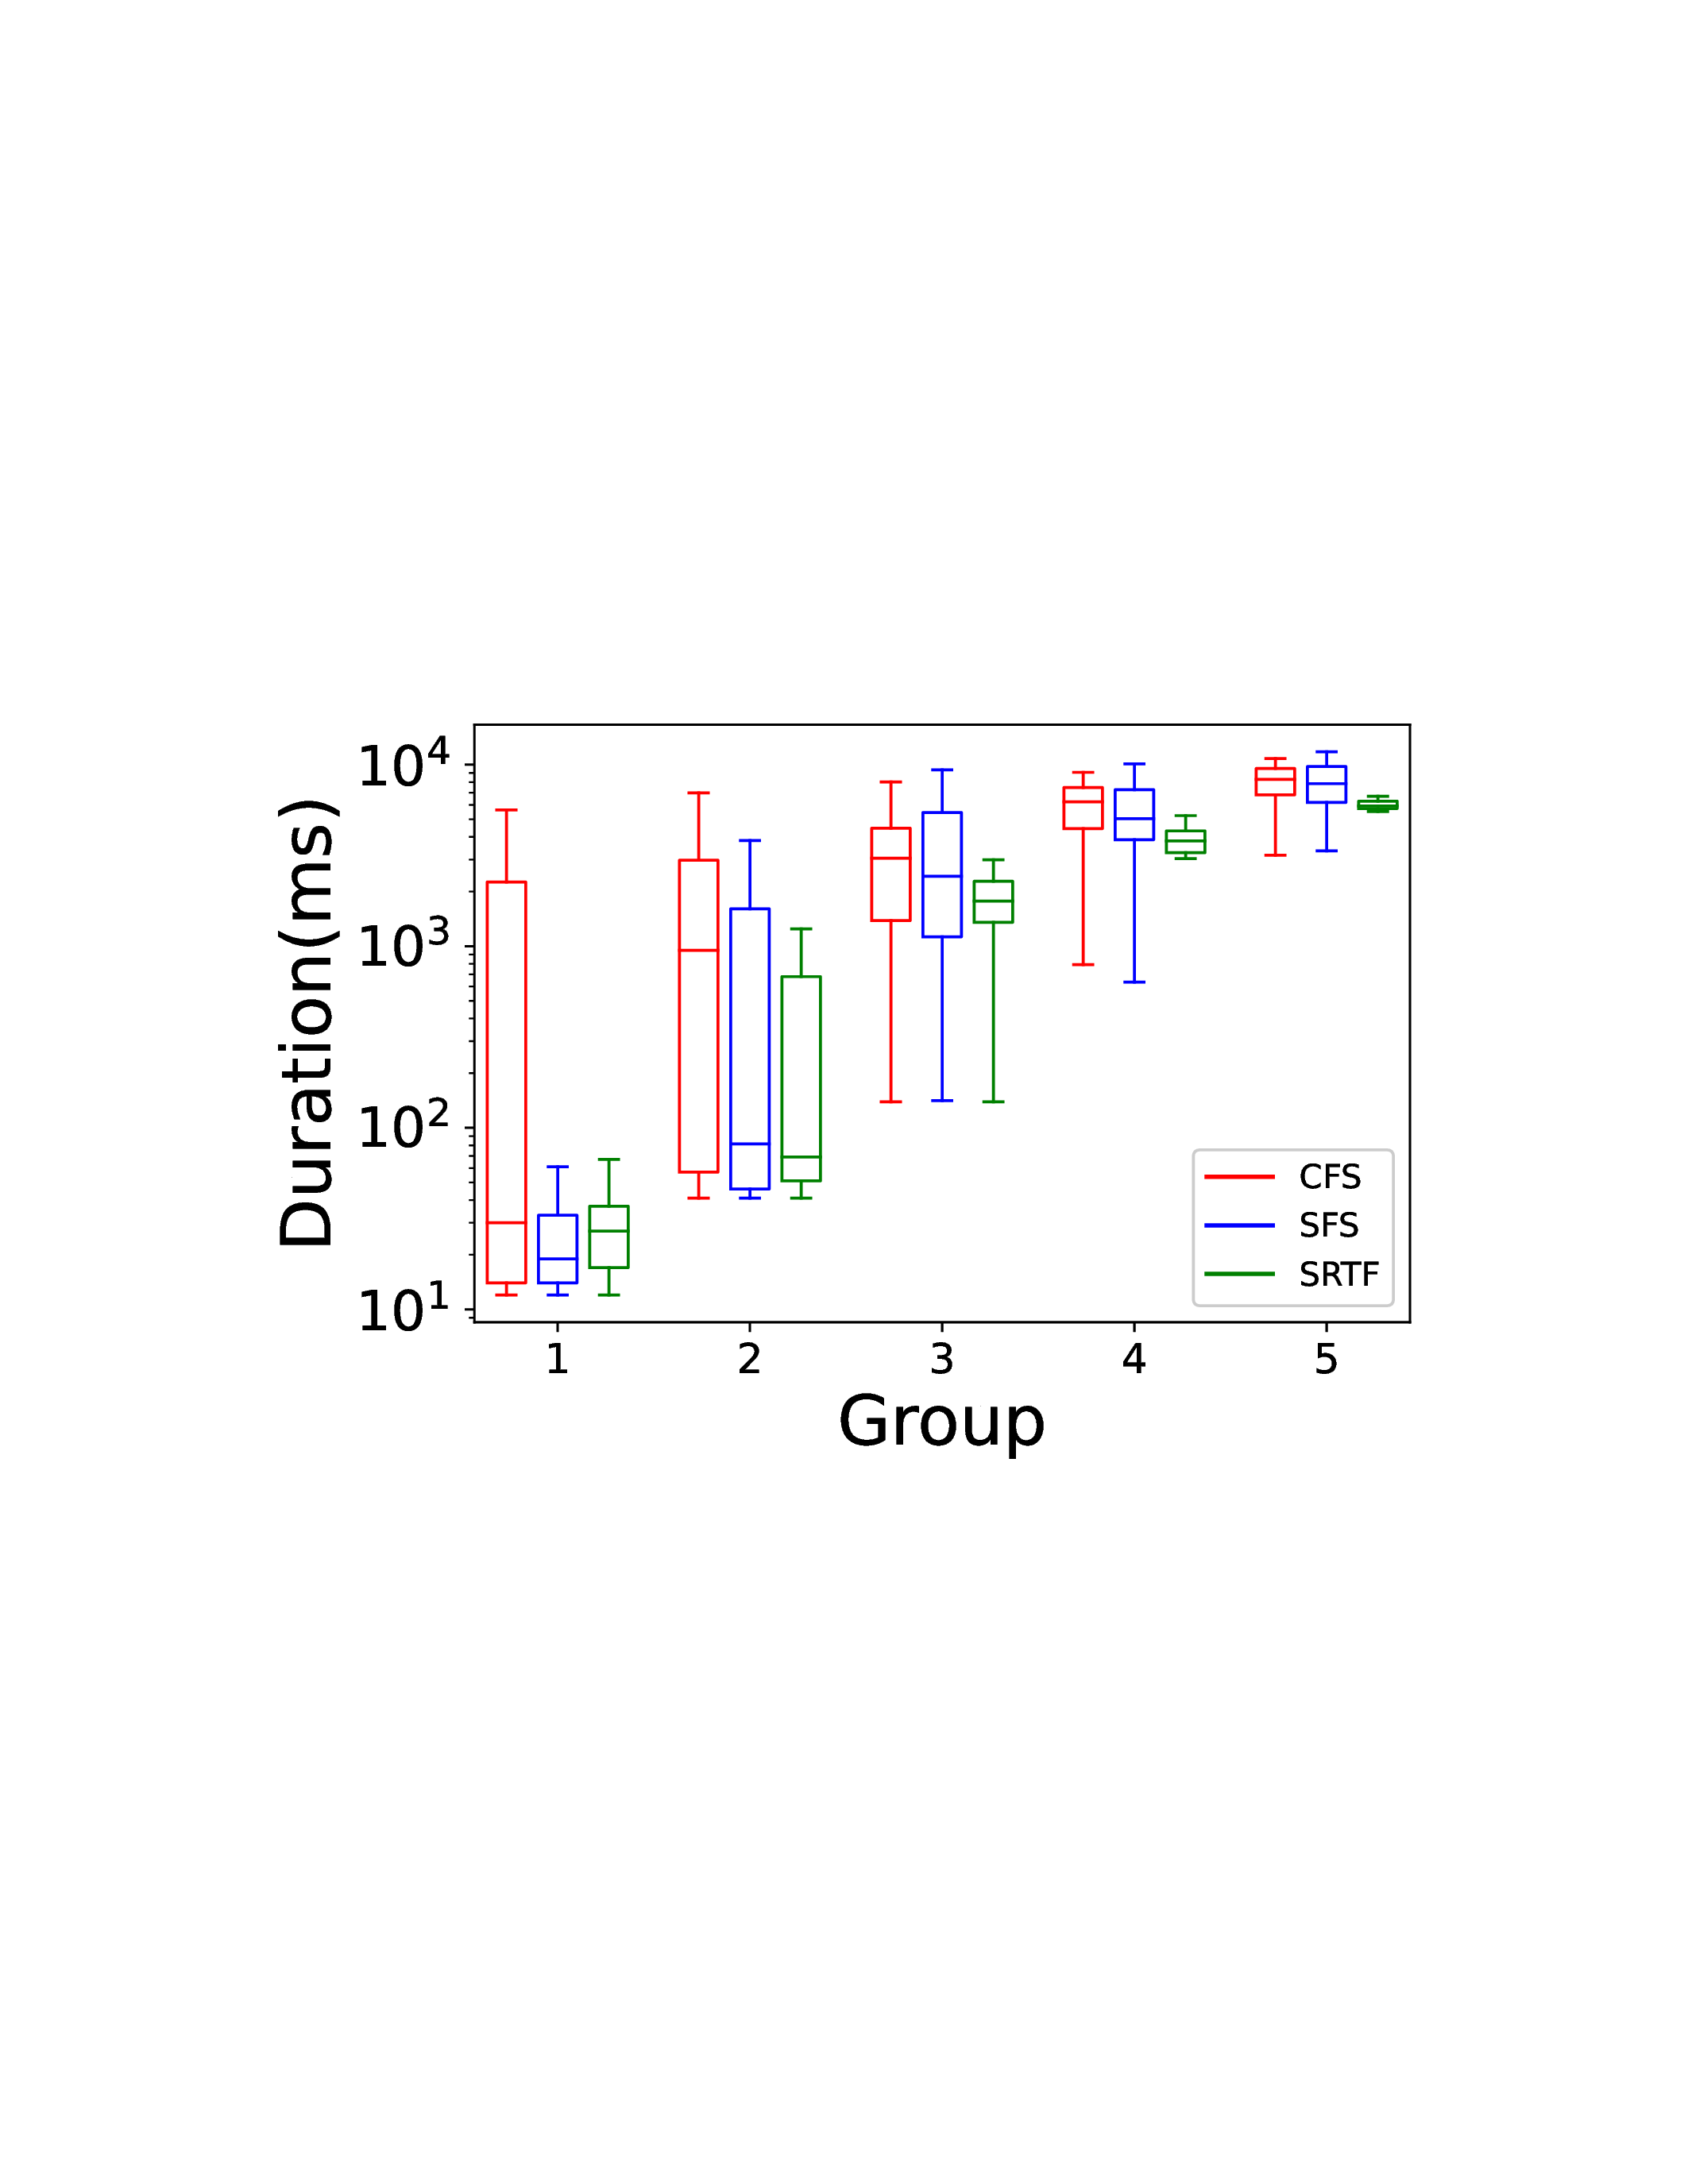}
\label{fig:short_box}
}
\hspace{-9pt}
\subfigure[Long-dominant.] {
\includegraphics[width=.23\textwidth]{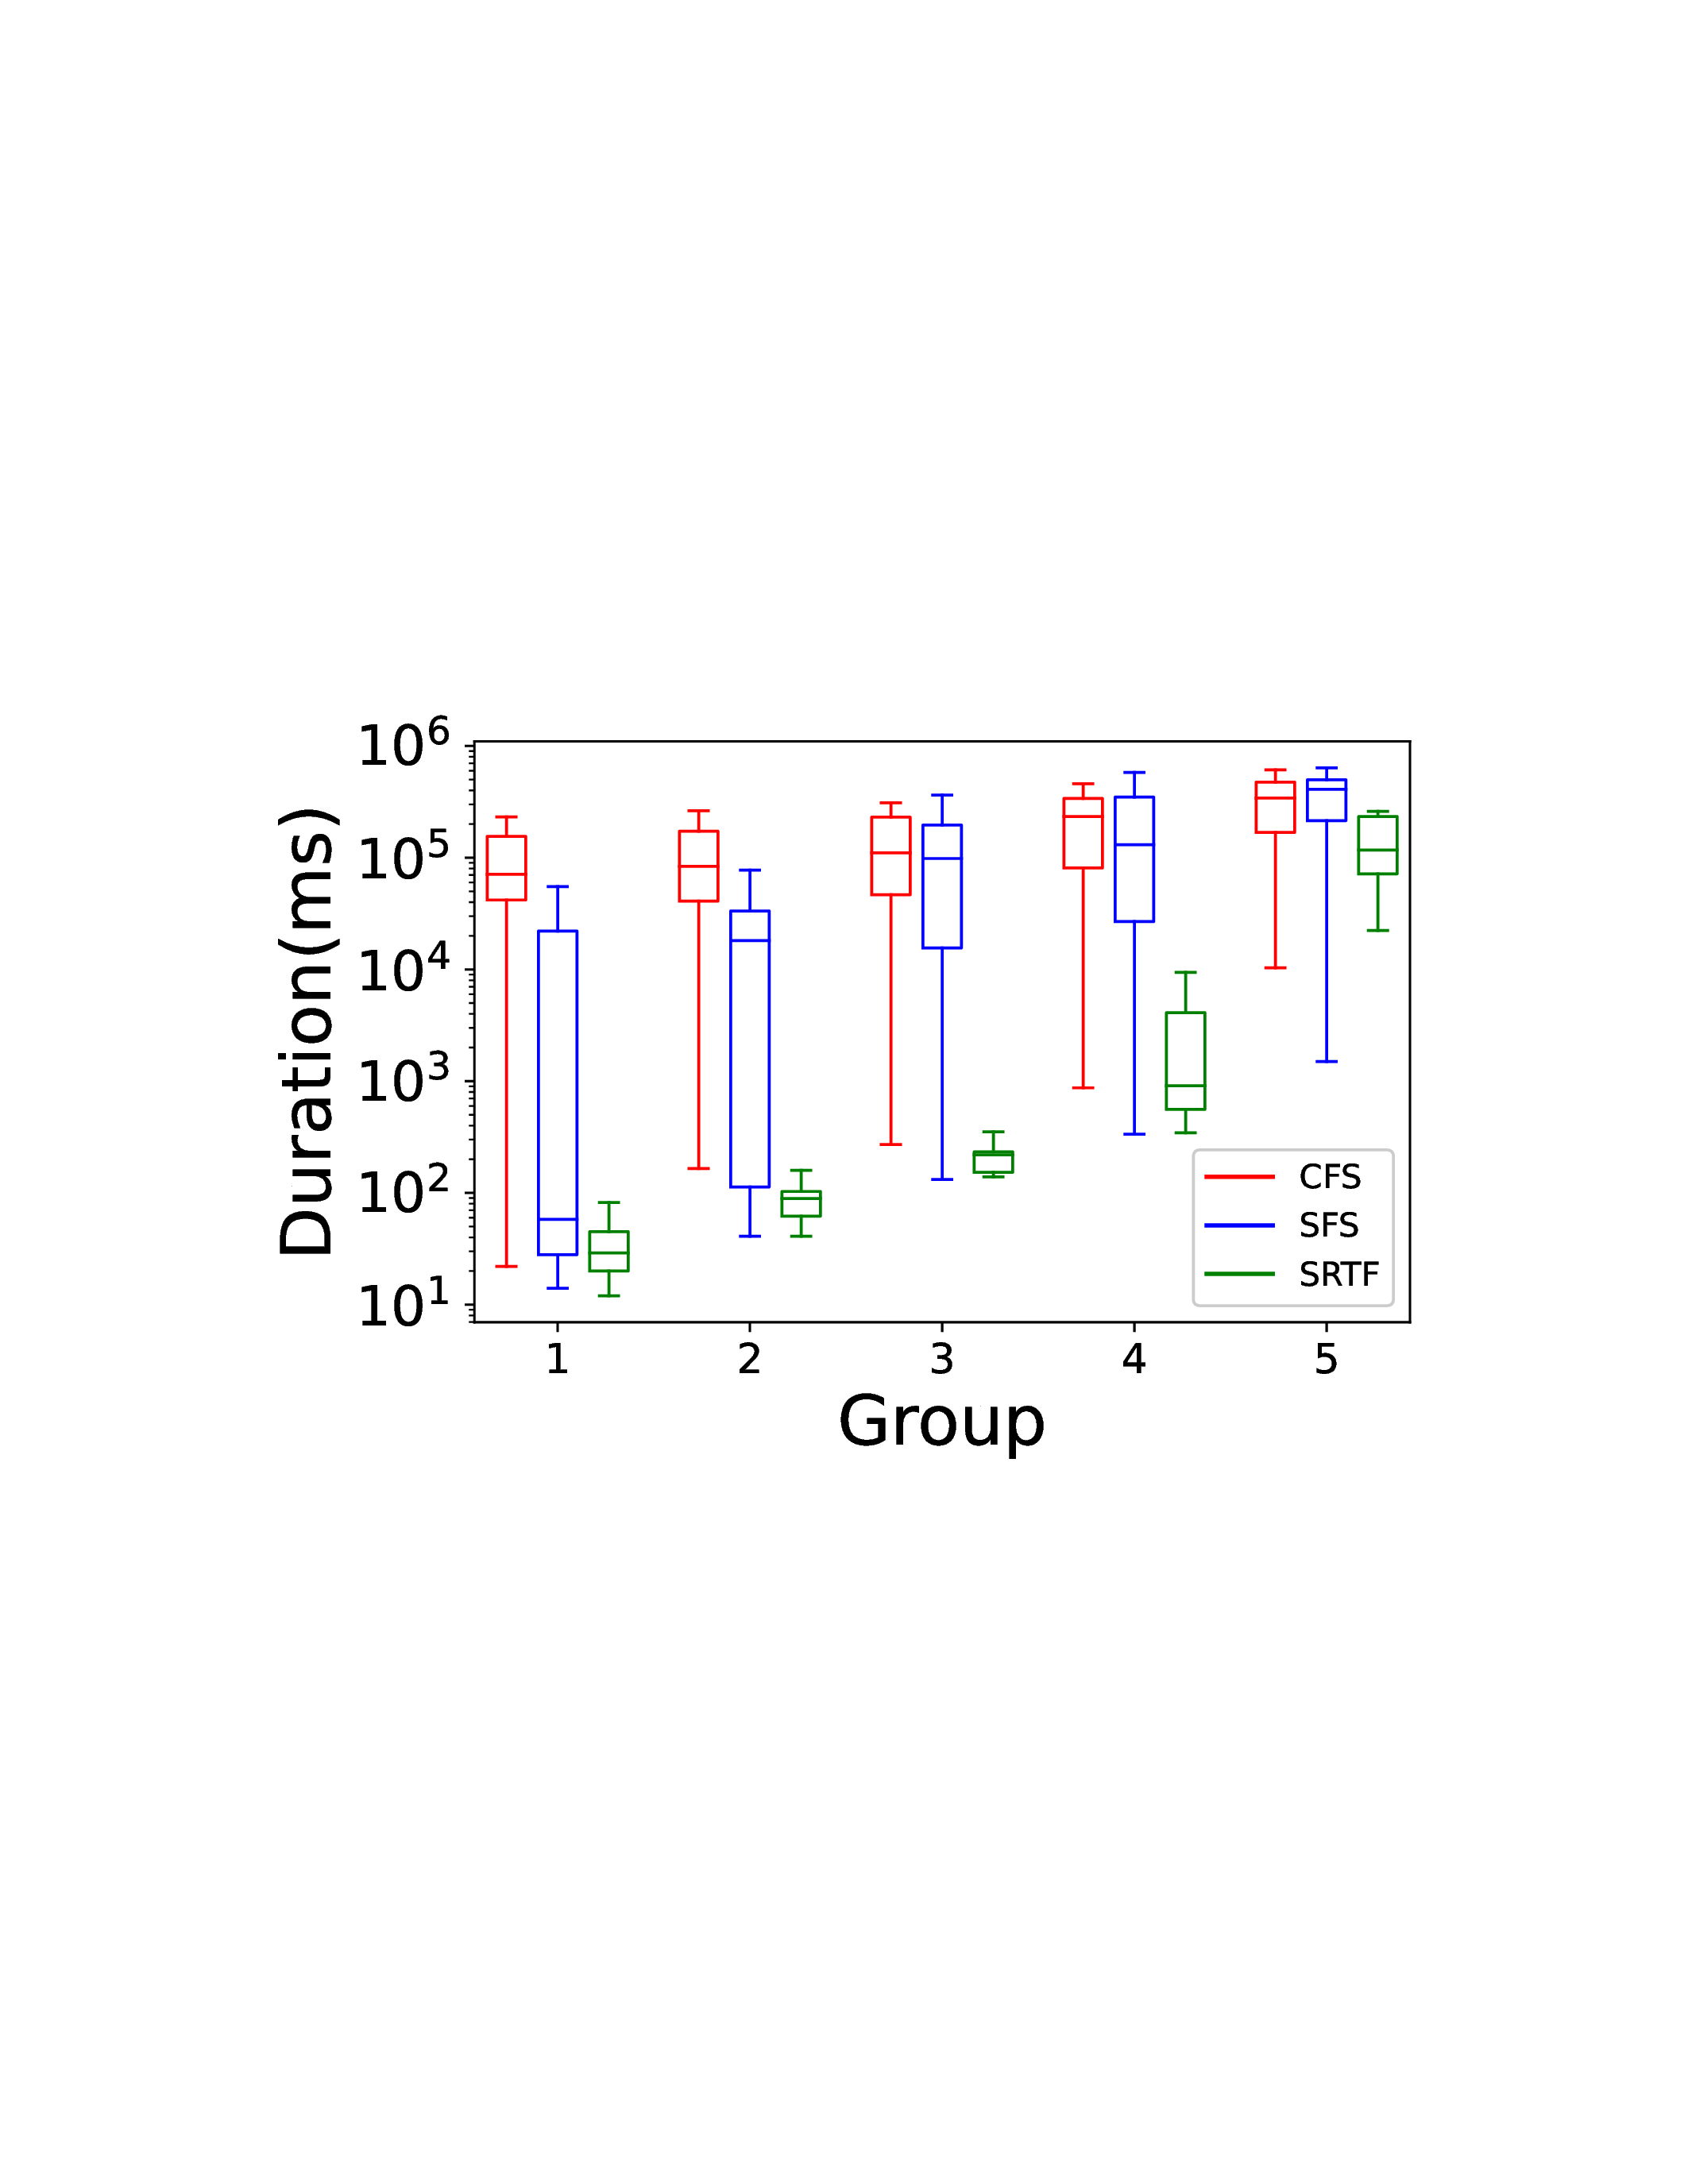}
\label{fig:long_box}
}
\hspace{-9pt}
\subfigure[Uniform.] {
\includegraphics[width=.23\textwidth]{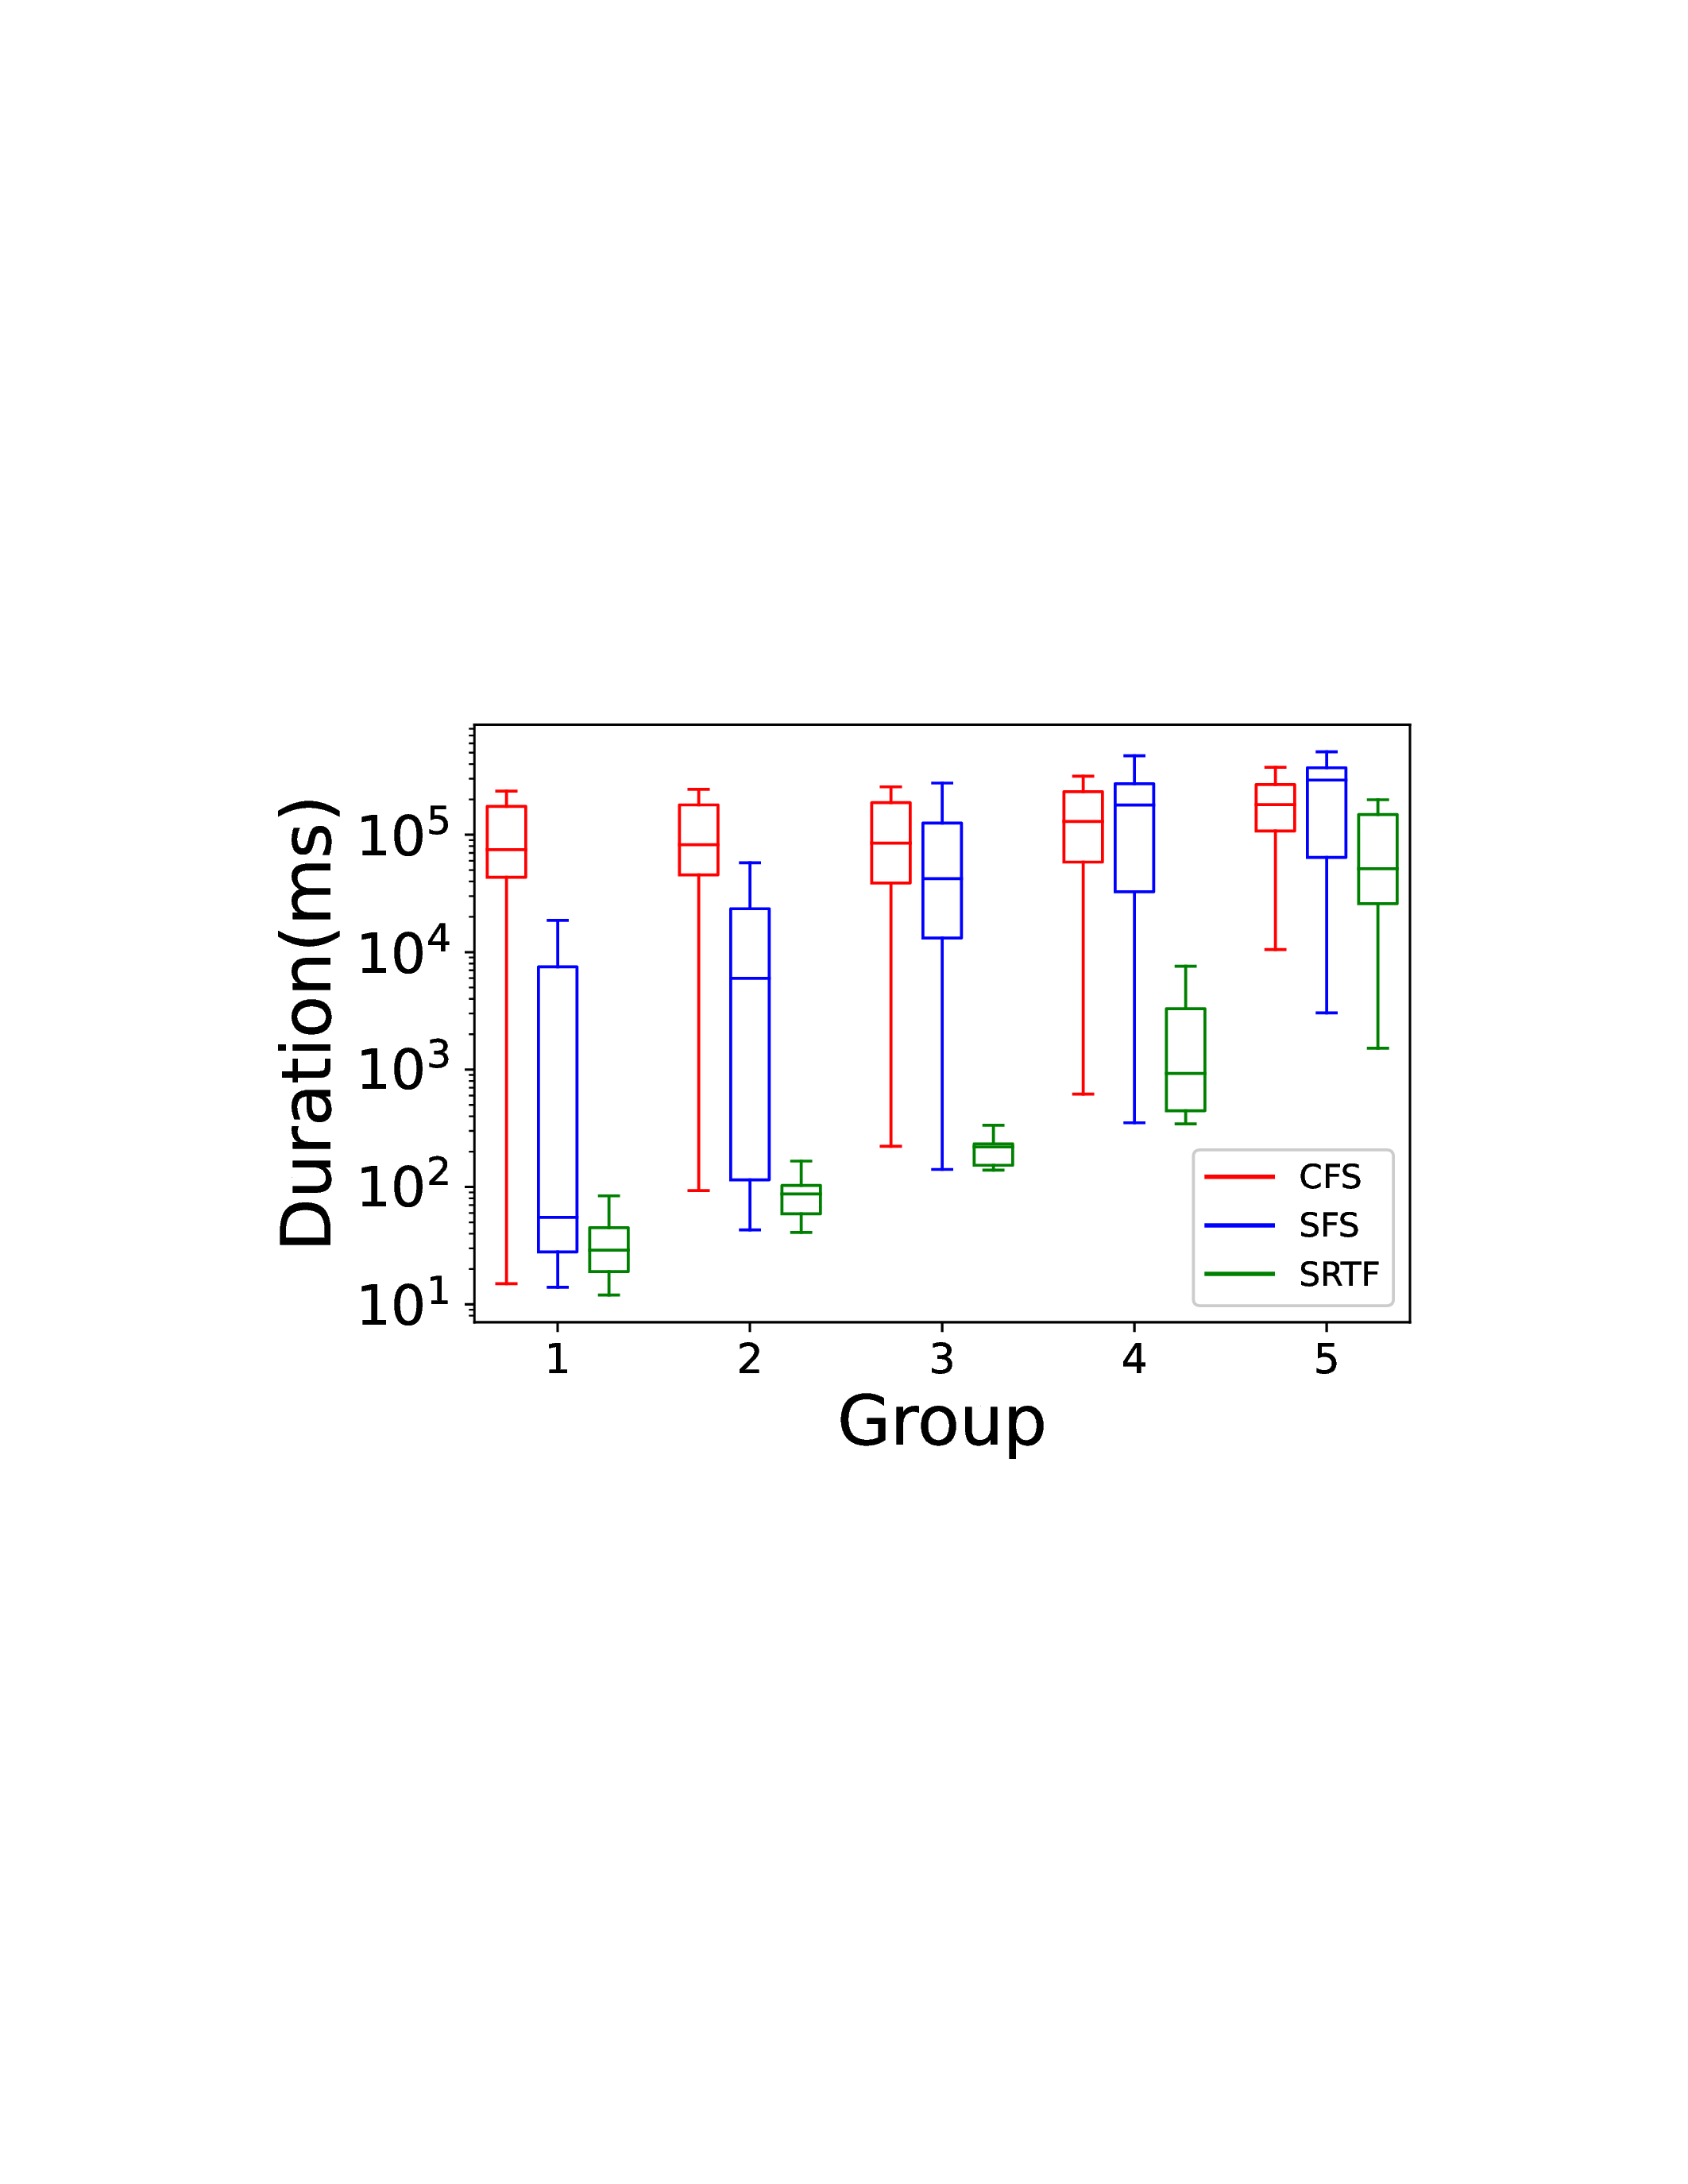}
\label{fig:unif_box}
}
\vspace{-10pt}
\caption{Performance distribution of different workloads derived from the Azure function trace. 
Figure~\ref{fig:azure_cdf}-\ref{fig:unif_cdf} plot the CDF of function duration.
Figure~\ref{fig:azure_box}-\ref{fig:unif_box} plot the box-and-whisker distributions of function duration
classified in five groups: groups are classified by the number of arithmetic operations (i.e., $N$s) of the {\fib} functions. 
Lower bound and upper bound of the box-whisker plots: $Q1 - 1.5 * IQR$ ($0.35^{th}$ percentile) and $Q3 + 1.5 * IQR$ ($99.65^{th}$ percentile). 
}
\label{fig:standalone_wl}
\end{center}
\vspace{-15pt}
\end{figure*}

\subsection{{\proj} Efficacy under Diverse Workloads}
\label{subsec:workload}
\vspace{-2pt}

\added{
We stress-test {\proj} using various high-load FaaS workloads 
%generated by {\bench} 
to understand how much better {\proj} can perform against CFS under different workload scenarios.}
We used {\bench} to generate four workloads.
%with different function duration distributions: 
In addition to the \emph{Azure-sampled workload} that follows the distribution of Azure traces (\cref{sec:methodology}), 
we used {\bench} to generate three other workloads:
%\emph{Azure workload} that follows the distribution of Azure function traces (\cref{sec:methodology});
\emph{Short-dominant workload}, where $80\%$ of the function invocations have an execution duration shorter than 50~ms;
\emph{Long-dominant workload}, where $20\%$ of the function invocations have an execution duration shorter than 50~ms;
and \emph{uniform workload}, where functions are uniformed drawn from each duration group.

%Figure~\ref{fig:standalone_wl} reports the detailed results. 
For each workload, we ran SRTF as the optimal case. We observe that {\proj} outperformed CFS for all workloads. Specifically, $44.4\%$ of function requests finished within 1~second under {\proj}, as shown in Figure~\ref{fig:azure_cdf}.  
%whereas only \yuec{YYY\%} of requests finish 
CFS had only $0.8\%$ of requests finished in 1~second. Worse, the $41^{th}$ percentile duration of CFS is $92\times$ longer than that of {\proj} due to CFS' fine-grained time-sharing and long scheduling cycles. 
The medium
%and $75^{th}$ percentile }
%average 
turnaround time of the first two groups' function invocations under {\proj} is \added{$216\times$ and $113\times$} faster than that of CFS (Figure~\ref{fig:azure_box}), respectively. 
%This demonstrates the effectiveness of {\proj} in optimizing short function turnaround time. 

%%%%%%%%%%%%%%%%%% varying slices

{\proj} is superior under short-dominant workloads as well. In fact, {\proj} approaches the optimal SRTF for $70\%$ of the requests (Figure~\ref{fig:short_cdf}). Recall, $80\%$ requests of the short-dominant workload could finish in 50~ms if running in an ideal environment without contention (Table~\ref{tbl:map}). Group~1 under {\proj}, covering a {\fib} $N$ of 20-26, had a median ($75^{th}$ percentile) duration of 19~ms (33~ms), whereas the same group of function requests observed dramatically larger duration variance  
%{\bf to be confirmed} 
under CFS (Figure~\ref{fig:short_box}). This once again showcases the optimality of {\proj} when handling short functions. 
%{\bf look at the box figure, for uniform, SFS is not better. Probably to differentiate the overall (CDF) results from group results? }

%{\proj} observed similar trends for long-dominant and uniform workloads, as shown in Figure~\ref{fig:long_cdf}-\ref{fig:unif_cdf} and \ref{fig:long_box}-\ref{fig:unif_box}. 
{\proj} achieved similar performance for long functions in group~5 under the short-dominant workload and long-dominant workload. 
This is because,
in both two scenarios, 
%long jobs received almost same service under both {\proj} and CFS--
long jobs are long enough that they receive almost the same amount of service (either too small under small-dominant workload or too large for long-dominant workload), proportionally, under both {\proj} and CFS. 
Long functions in group~5 were marginally impacted in Azure-sampled workload and uniform workload, since the function duration distribution is more balanced and higher-priority, shorter functions ``steal'' service time from long functions, causing a slightly longer waiting time for them.
\fi
